# Supplementary material for: Janus van der Waals equations for real molecules with two-sided phase transitions
Source: arXiv:2204.05557 source file (2022-04-12)
Supplement: Supplementary file 1 [file frontiers_SupplementaryMaterial.pdf]

# Supplementary Material for “Janus van der Waals equations for real molecules with two-sided phase transitions”

Jihwan Kim, Do-Hyun Kim, and Jeong-Hyuck Park

## SM 1 SUPPLEMENTARY FIGURES FOR $N = 4$ CASE

### SM 1.1 argon (Ar)

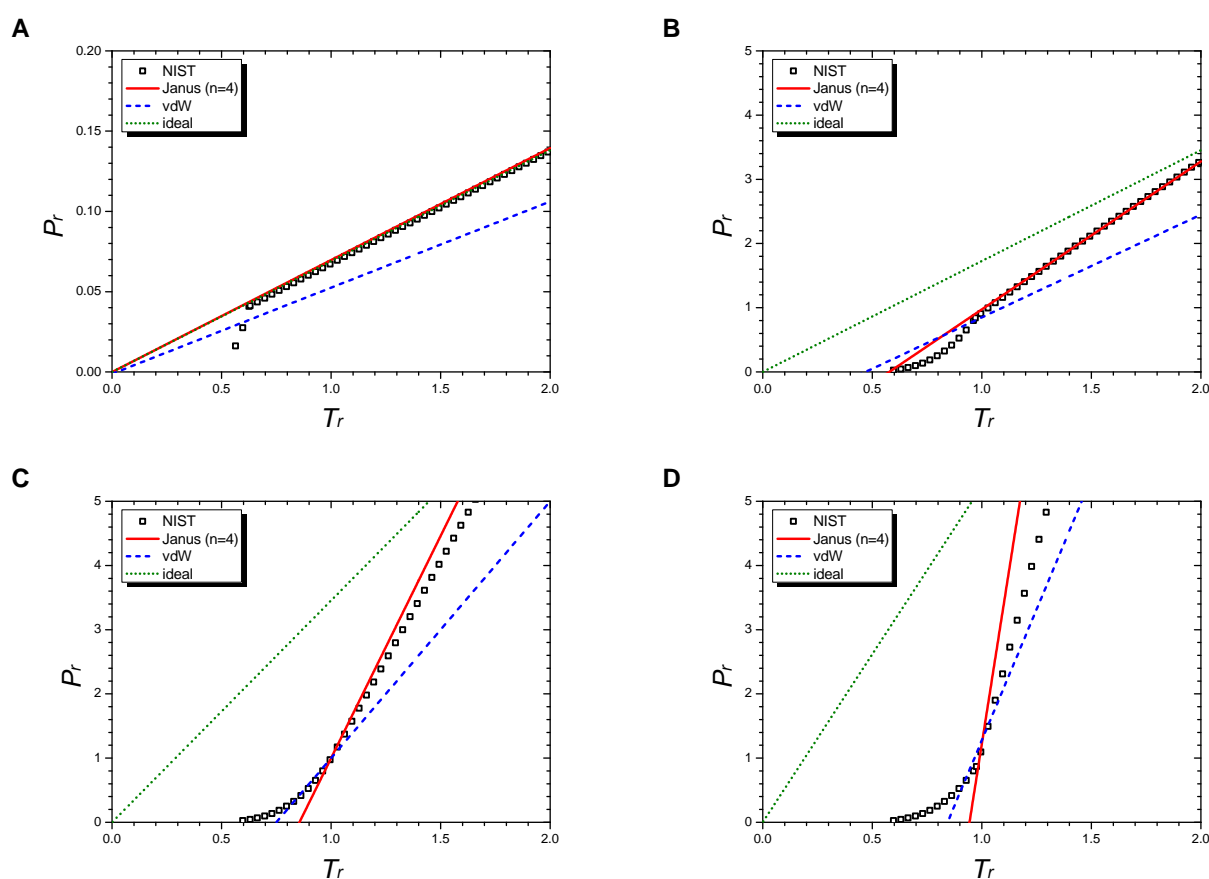

**Figure S1.** Isochoric curves of argon (Ar) at  $1/v_r = 0.02$  (A),  $1/v_r = 0.5$  (B),  $1/v_r = 1.0$  (C), and  $1/v_r = 1.5$  (D). Boxes are from the NIST data. The red solid line is drawn from the  $n = 4$  Janus van der Waals equation, the blue dashed line from the original van der Waals equation, and the green dotted line from the classical ideal gas law.

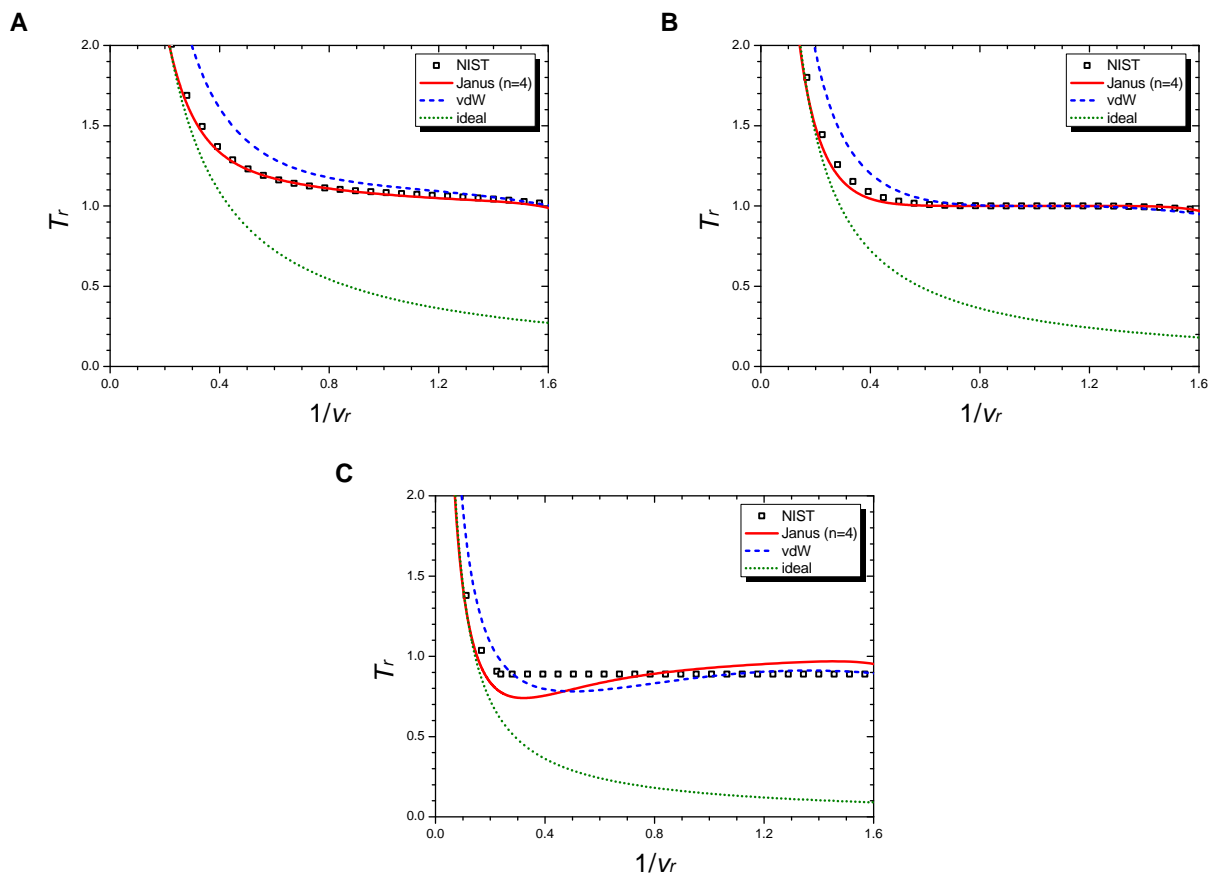

**Figure S2.** Isobaric curves of argon (Ar) at  $P_r = 1.5$  (A),  $P_r = 1.0$  (B), and  $P_r = 0.5$  (C). Boxes are from the NIST data. The red solid line is drawn from the  $n = 4$  Janus van der Waals equation, the blue dashed line from the original van der Waals equation, and the green dotted line from the classical ideal gas law.

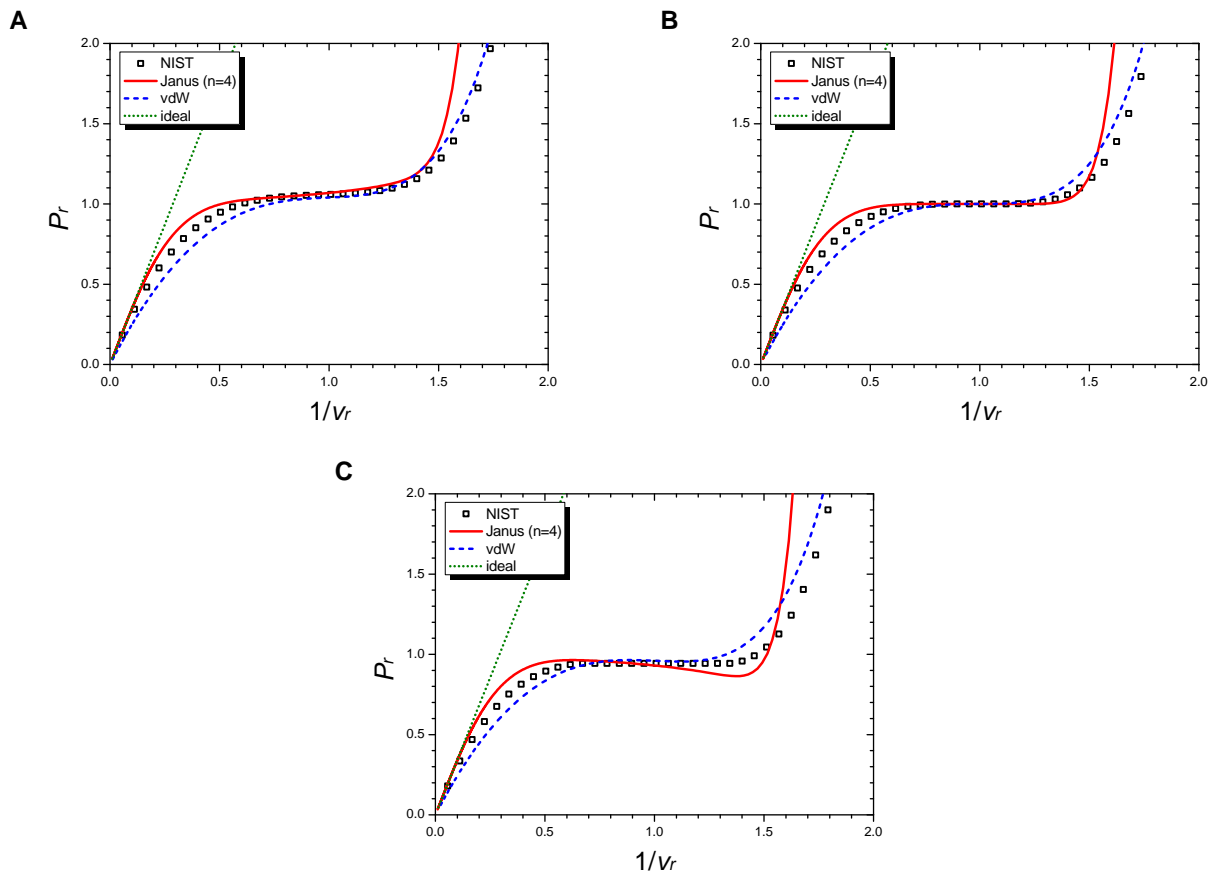

**Figure S3.** Isothermal curves of argon (Ar) at  $T_r = 1.01$  (A),  $T_r = 1.00$  (B), and  $T_r = 0.99$  (C). Boxes are from the NIST data. The red solid line is drawn from the  $n = 4$  Janus van der Waals equation, the blue dashed line from the original van der Waals equation, and the green dotted line from the classical ideal gas law.

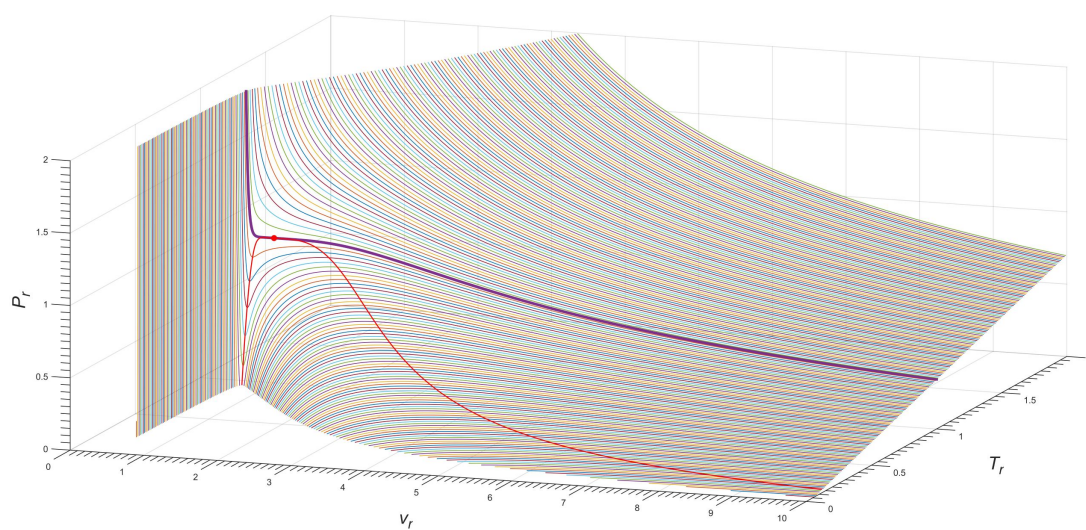

**Figure S4.** Three-dimensional  $P_r - v_r - T_r$  phase diagram of the exact  $n = 4$  Janus van der Waals equation, as for argon (Ar). The bold purple line corresponds to the isotherm of  $T_r = 1.00$  as depicted in **Figure S3 B**; the red line is the Janus van der Waals spinodal curve with  $a = 0.99$ ; and the red dot is the critical point.



SM 1.2 methane ( $\text{CH}_4$ )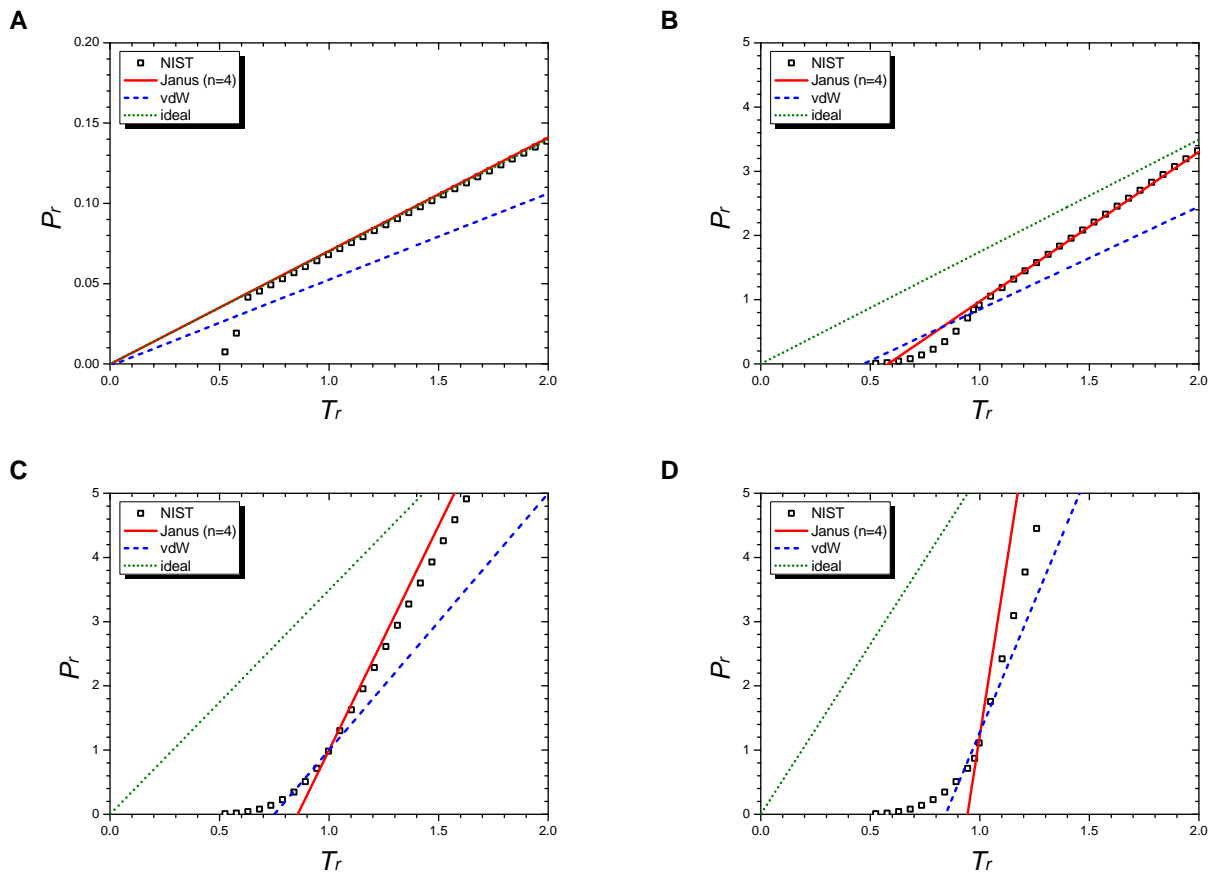

**Figure S5.** Isochoric curves of methane ( $\text{CH}_4$ ) at  $1/v_r = 0.02$  (A),  $1/v_r = 0.5$  (B),  $1/v_r = 1.0$  (C), and  $1/v_r = 1.5$  (D). Boxes are from the NIST data. The red solid line is drawn from the  $n = 4$  Janus van der Waals equation, the blue dashed line from the original van der Waals equation, and the green dotted line from the classical ideal gas law.

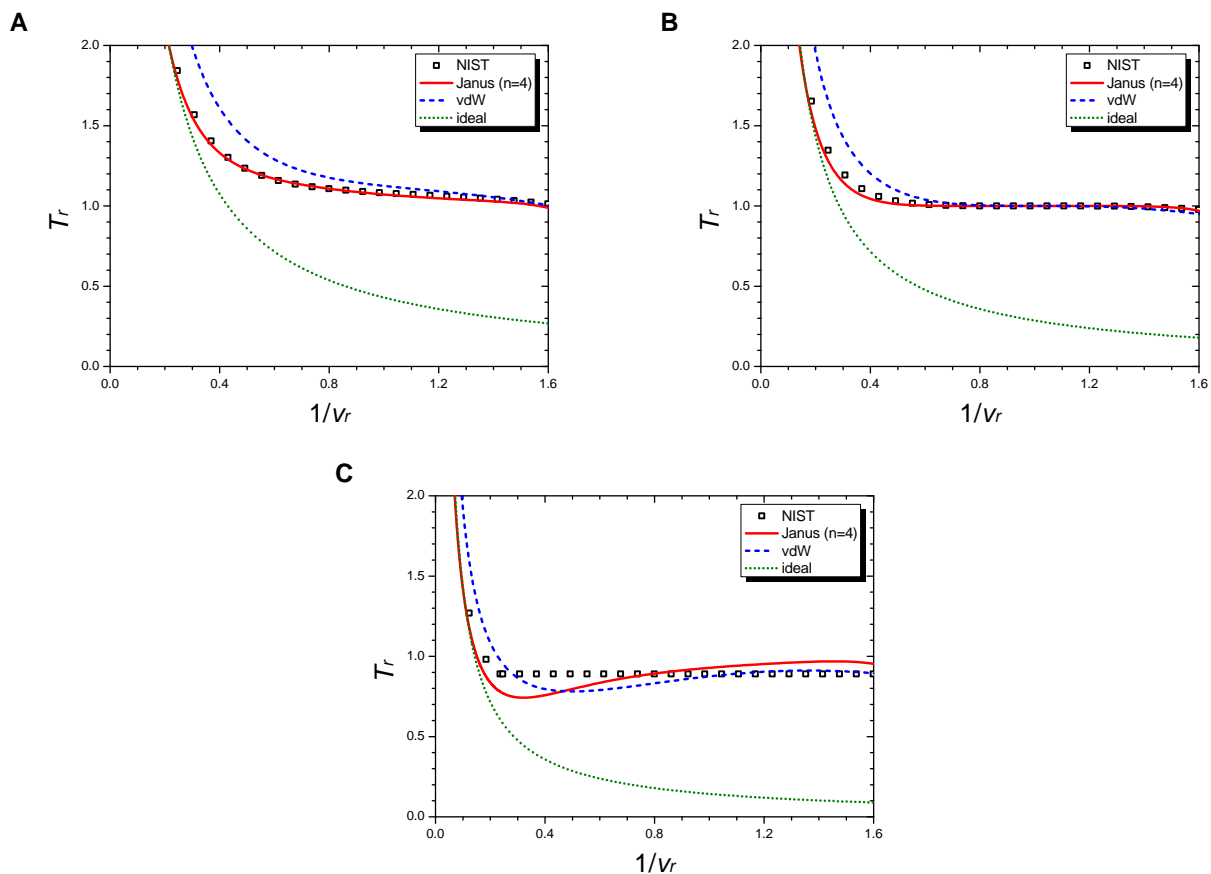

**Figure S6.** Isobaric curves of methane ( $\text{CH}_4$ ) at  $P_r = 1.5$  (A),  $P_r = 1.0$  (B), and  $P_r = 0.5$  (C). Boxes are from the NIST data. The red solid line is drawn from the  $n = 4$  Janus van der Waals equation, the blue dashed line from the original van der Waals equation, and the green dotted line from the classical ideal gas law.

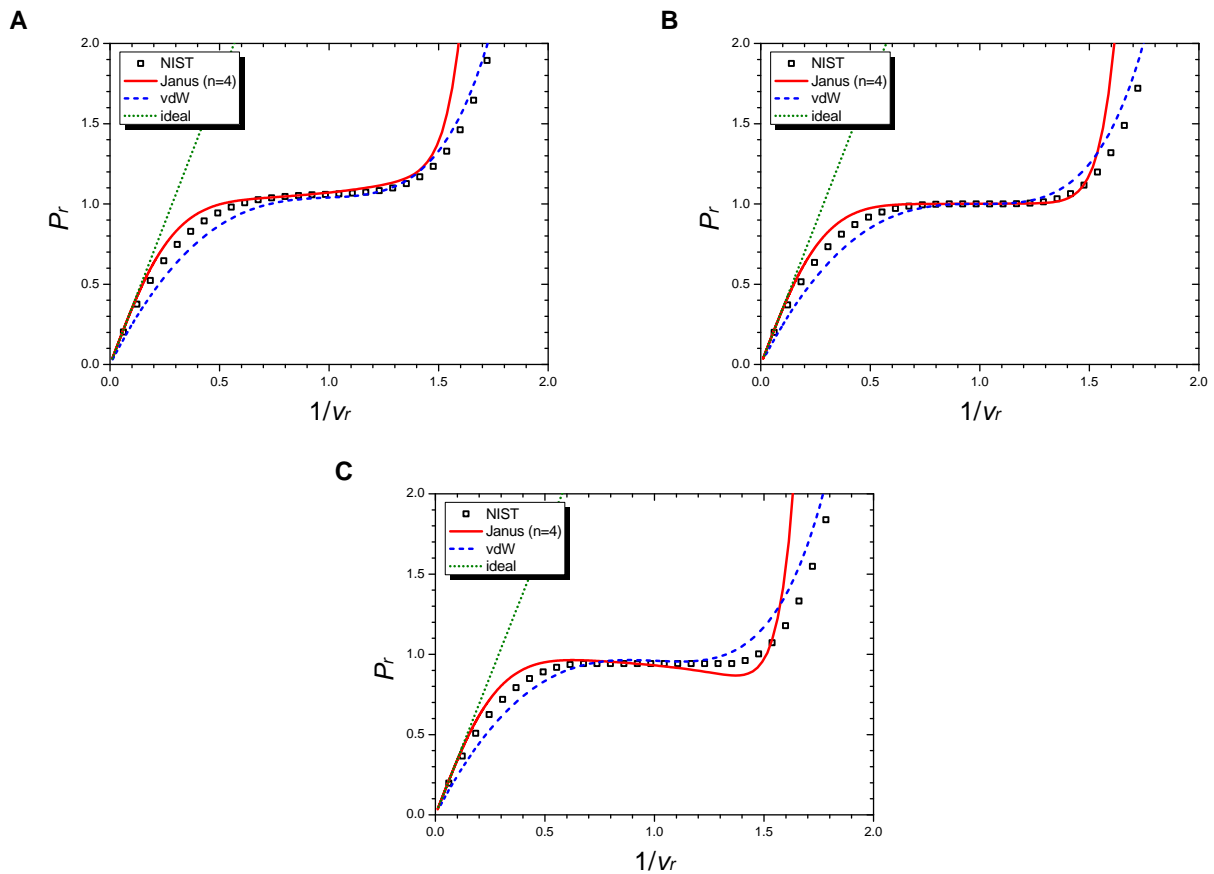

**Figure S7.** Isothermal curves of methane ( $\text{CH}_4$ ) at  $T_r = 1.01$  (A),  $T_r = 1.00$  (B), and  $T_r = 0.99$  (C). Boxes are from the NIST data. The red solid line is drawn from the  $n = 4$  Janus van der Waals equation, the blue dashed line from the original van der Waals equation, and the green dotted line from the classical ideal gas law.

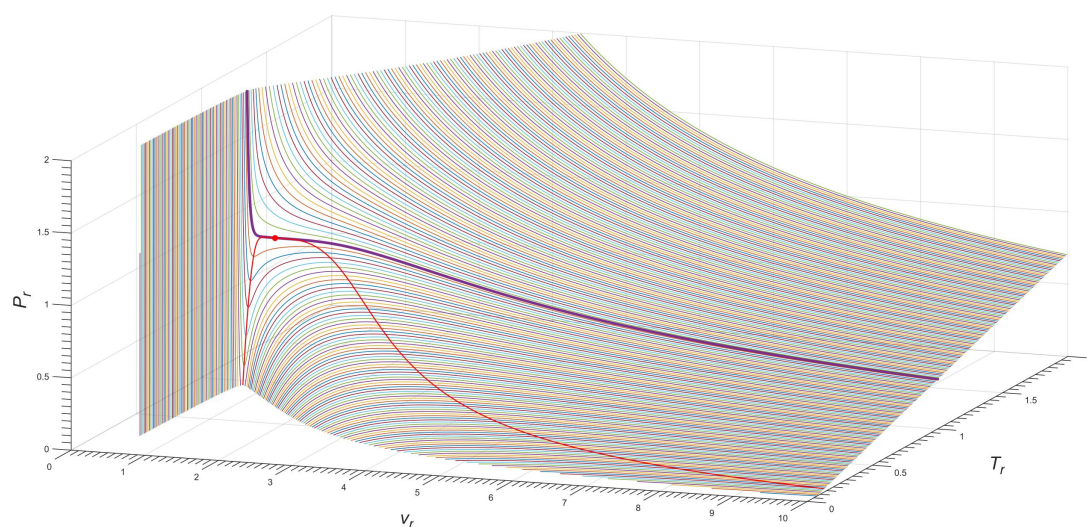

**Figure S8.** Three-dimensional  $P_r - v_r - T_r$  phase diagram of the exact  $n = 4$  Janus van der Waals equation, as for methane ( $\text{CH}_4$ ). The bold purple line corresponds to the isotherm of  $T_r = 1.00$  as depicted in **Figure S7 B**; the red line is the Janus van der Waals spinodal curve with  $a = 0.99$ ; and the red dot is the critical point.

SM 1.3 ethylene ( $\text{C}_2\text{H}_4$ )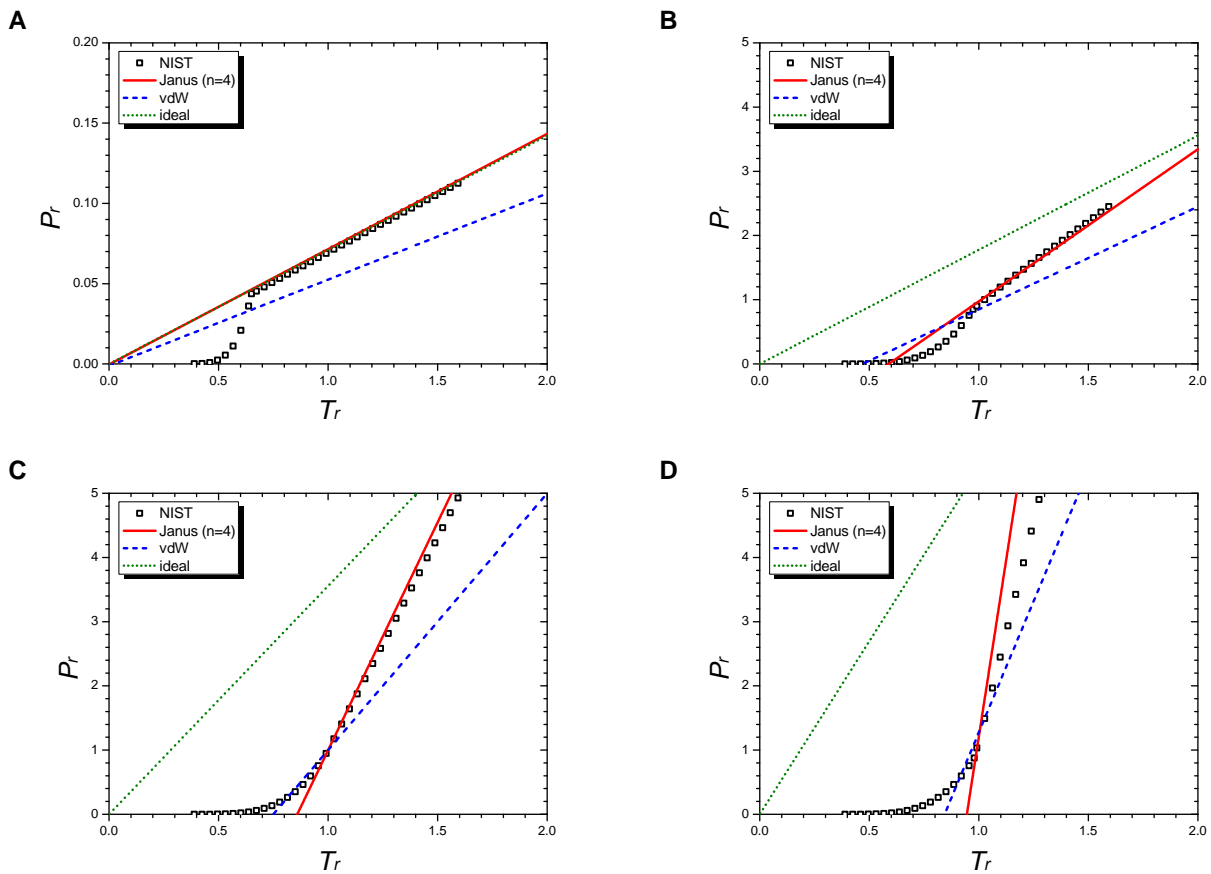

**Figure S9.** Isochoric curves of ethylene ( $\text{C}_2\text{H}_4$ ) at  $1/v_r = 0.02$  (A),  $1/v_r = 0.5$  (B),  $1/v_r = 1.0$  (C), and  $1/v_r = 1.5$  (D). Boxes are from the NIST data. The red solid line is drawn from the  $n = 4$  Janus van der Waals equation, the blue dashed line from the original van der Waals equation, and the green dotted line from the classical ideal gas law.

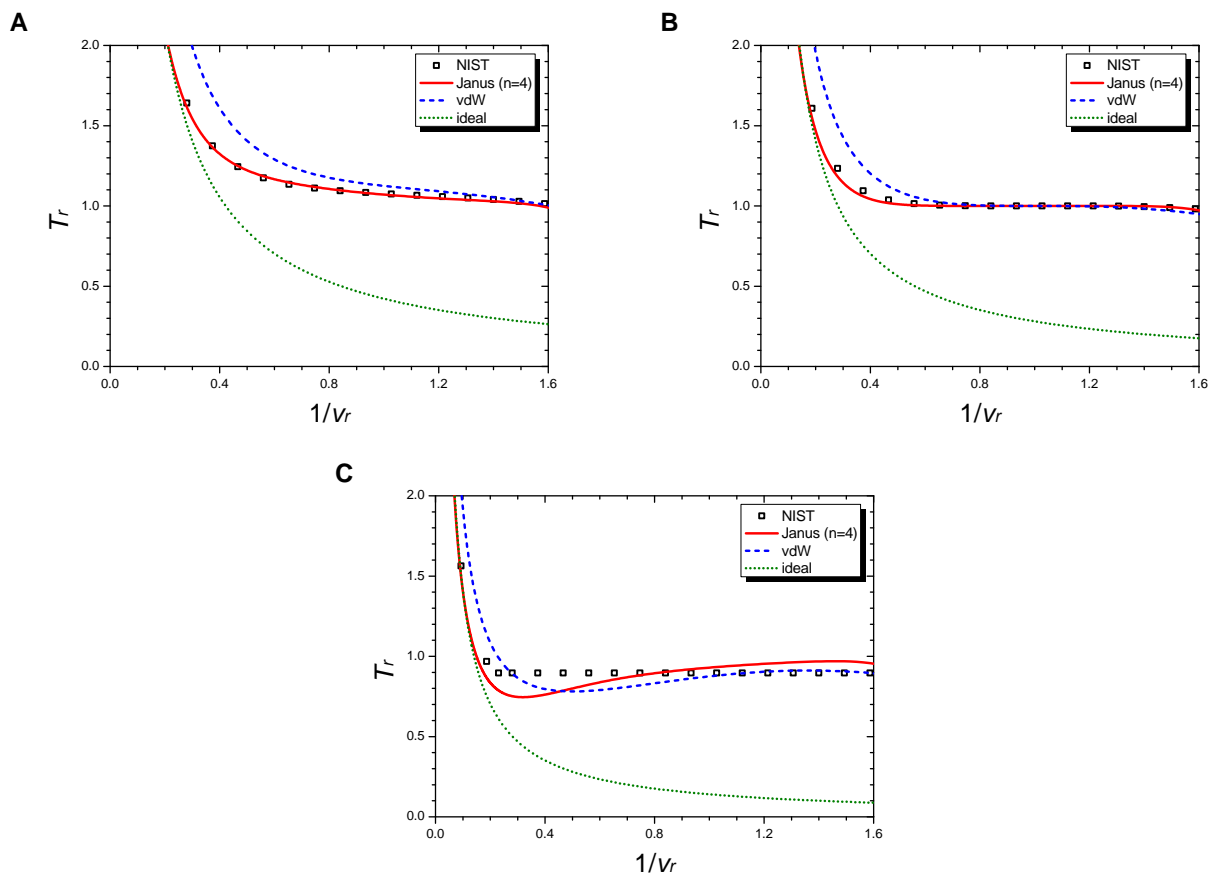

**Figure S10.** Isobaric curves of ethylene ( $\text{C}_2\text{H}_4$ ) at  $P_r = 1.5$  (A),  $P_r = 1.0$  (B), and  $P_r = 0.5$  (C). Boxes are from the NIST data. The red solid line is drawn from the  $n = 4$  Janus van der Waals equation, the blue dashed line from the original van der Waals equation, and the green dotted line from the classical ideal gas law.

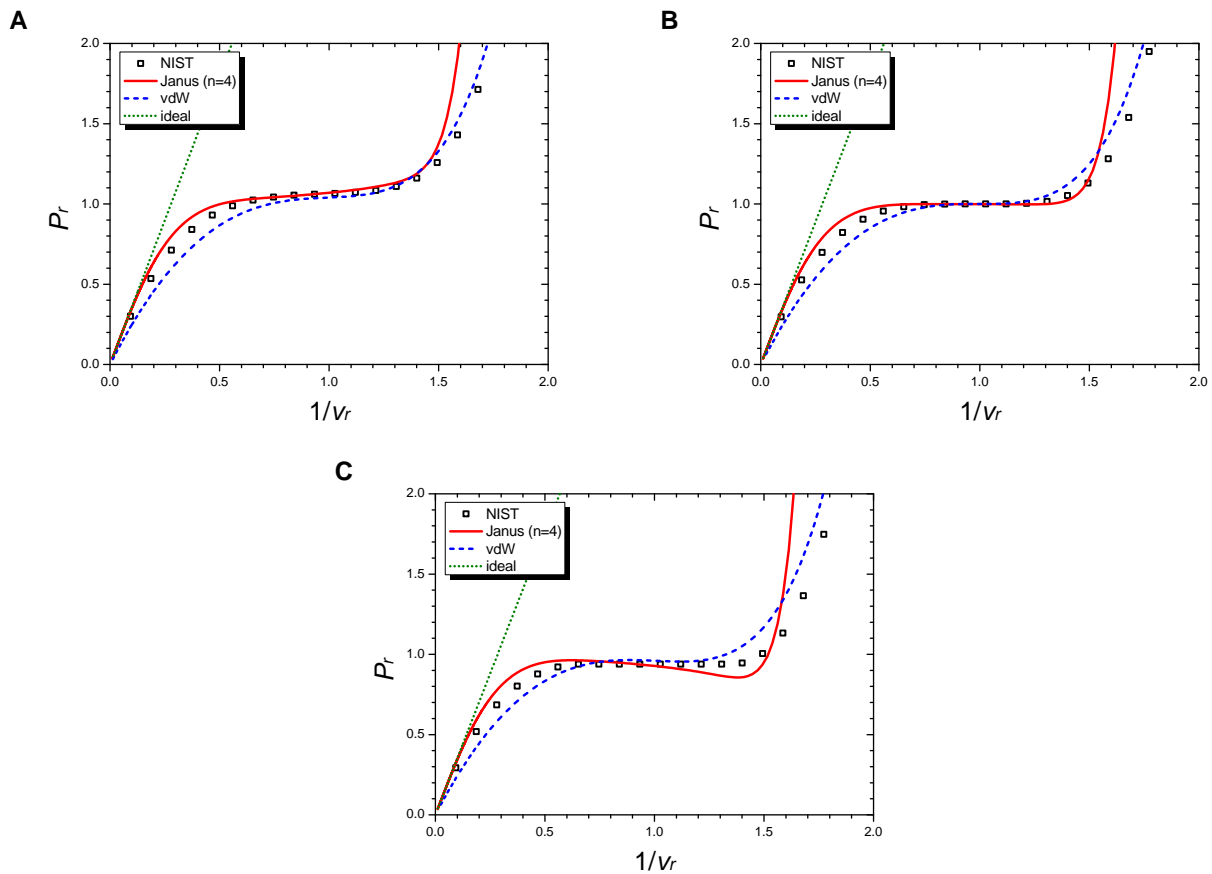

**Figure S11.** Isothermal curves of ethylene ( $C_2H_4$ ) at  $T_r = 1.01$  (A),  $T_r = 1.00$  (B), and  $T_r = 0.99$  (C). Boxes are from the NIST data. The red solid line is drawn from the  $n = 4$  Janus van der Waals equation, the blue dashed line from the original van der Waals equation, and the green dotted line from the classical ideal gas law.

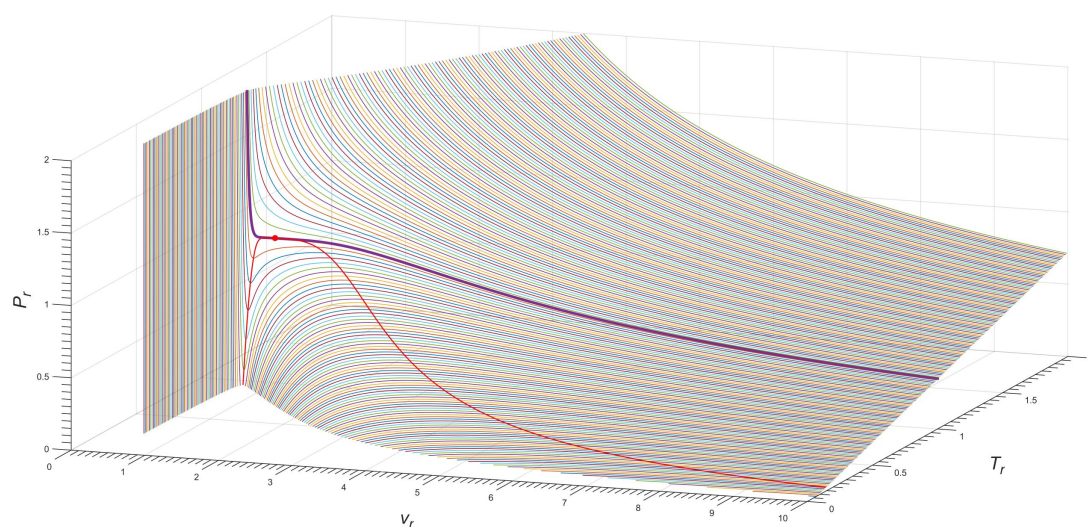

**Figure S12.** Three-dimensional  $P_r - v_r - T_r$  phase diagram of the exact  $n = 4$  Janus van der Waals equation, as for ethylene ( $\text{C}_2\text{H}_4$ ). The bold purple line corresponds to the isotherm of  $T_r = 1.00$  as depicted in **Figure S11 B**; the red line is the Janus van der Waals spinodal curve with  $a = 0.99$ ; and the red dot is the critical point.



SM 1.4 ethane ( $\text{C}_2\text{H}_6$ )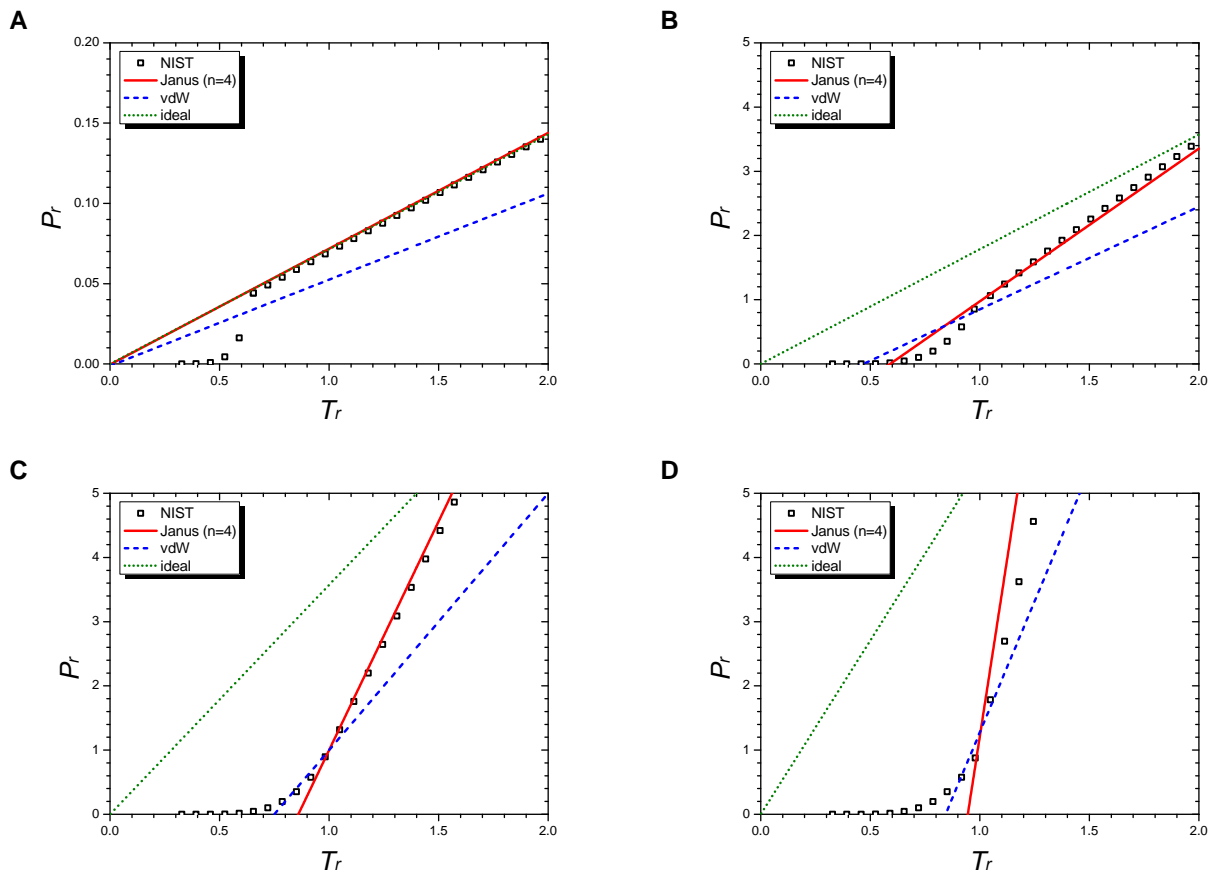

**Figure S13.** Isochoric curves of ethane ( $\text{C}_2\text{H}_6$ ) at  $1/v_r = 0.02$  (A),  $1/v_r = 0.5$  (B),  $1/v_r = 1.0$  (C), and  $1/v_r = 1.5$  (D). Boxes are from the NIST data. The red solid line is drawn from the  $n = 4$  Janus van der Waals equation, the blue dashed line from the original van der Waals equation, and the green dotted line from the classical ideal gas law.

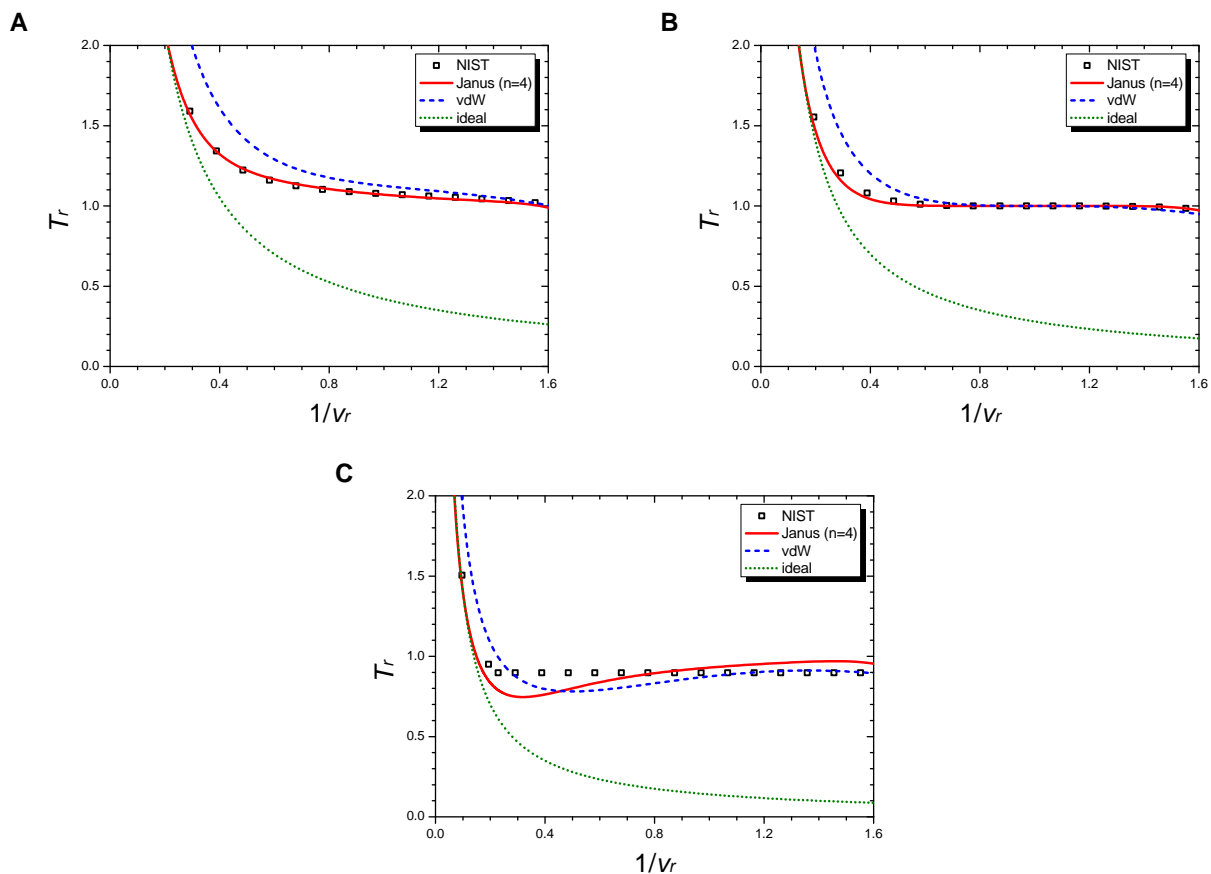

**Figure S14.** Isobaric curves of ethane ( $C_2H_6$ ) at  $P_r = 1.5$  (A),  $P_r = 1.0$  (B), and  $P_r = 0.5$  (C). Boxes are from the NIST data. The red solid line is drawn from the  $n = 4$  Janus van der Waals equation, the blue dashed line from the original van der Waals equation, and the green dotted line from the classical ideal gas law.

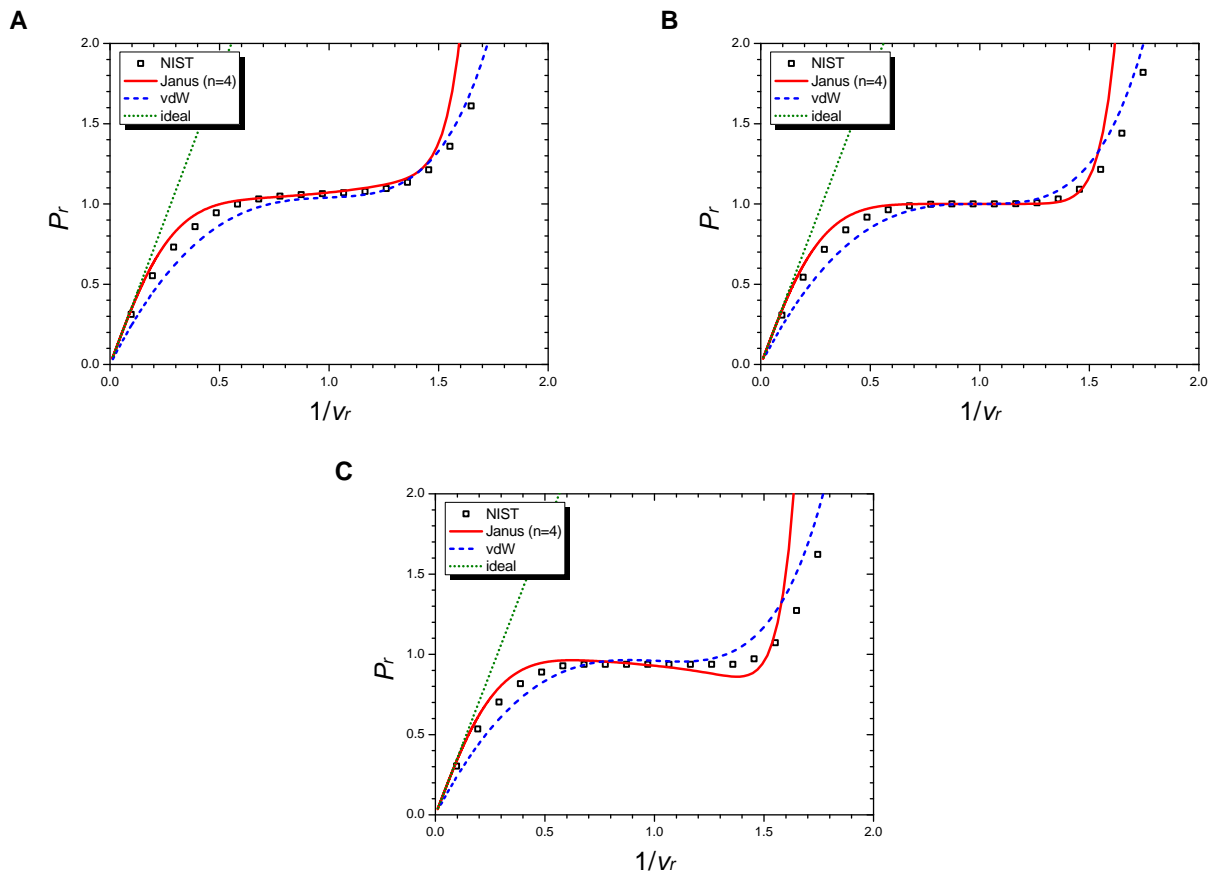

**Figure S15.** Isothermal curves of ethane ( $\text{C}_2\text{H}_6$ ) at  $T_r = 1.01$  (A),  $T_r = 1.00$  (B), and  $T_r = 0.99$  (C). Boxes are from the NIST data. The red solid line is drawn from the  $n = 4$  Janus van der Waals equation, the blue dashed line from the original van der Waals equation, and the green dotted line from the classical ideal gas law.

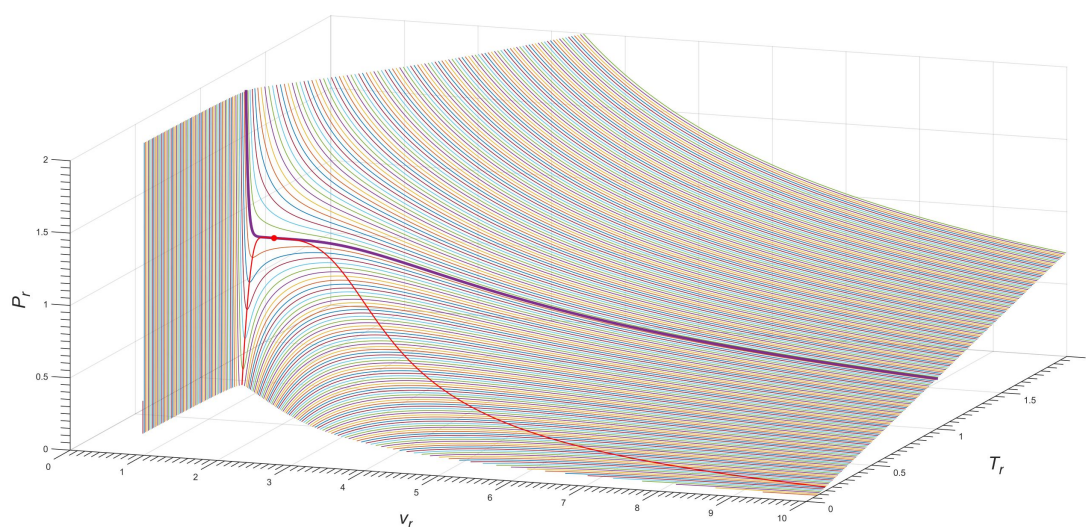

**Figure S16.** Three-dimensional  $P_r - v_r - T_r$  phase diagram of the exact  $n = 4$  Janus van der Waals equation, as for ethane ( $\text{C}_2\text{H}_6$ ). The bold purple line corresponds to the isotherm of  $T_r = 1.00$  as depicted in **Figure S15 B**; the red line is the Janus van der Waals spinodal curve with  $a = 0.99$ ; and the red dot is the critical point.

SM 1.5 propylene ( $\text{C}_3\text{H}_6$ )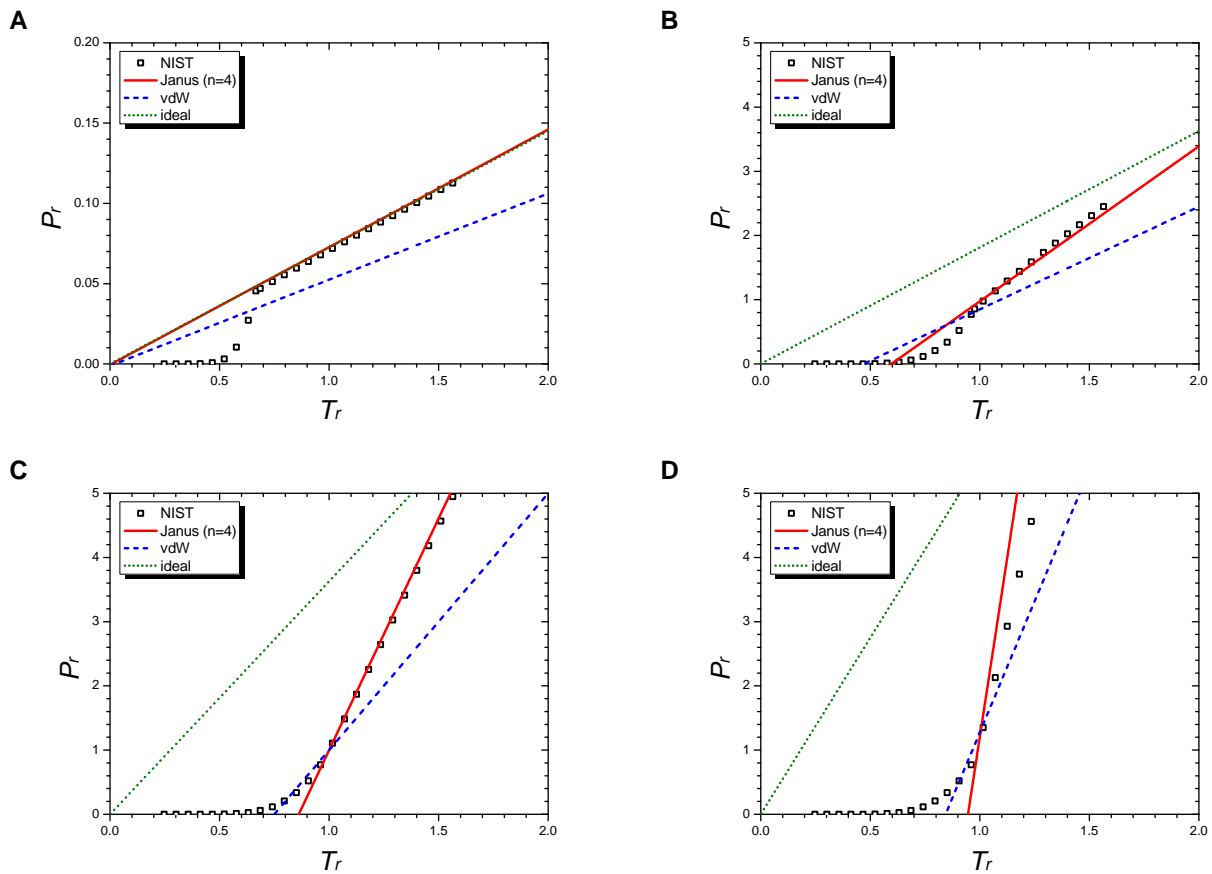

**Figure S17.** Isochoric curves of propylene ( $\text{C}_3\text{H}_6$ ) at  $1/v_r = 0.02$  (A),  $1/v_r = 0.5$  (B),  $1/v_r = 1.0$  (C), and  $1/v_r = 1.5$  (D). Boxes are from the NIST data. The red solid line is drawn from the  $n = 4$  Janus van der Waals equation, the blue dashed line from the original van der Waals equation, and the green dotted line from the classical ideal gas law.

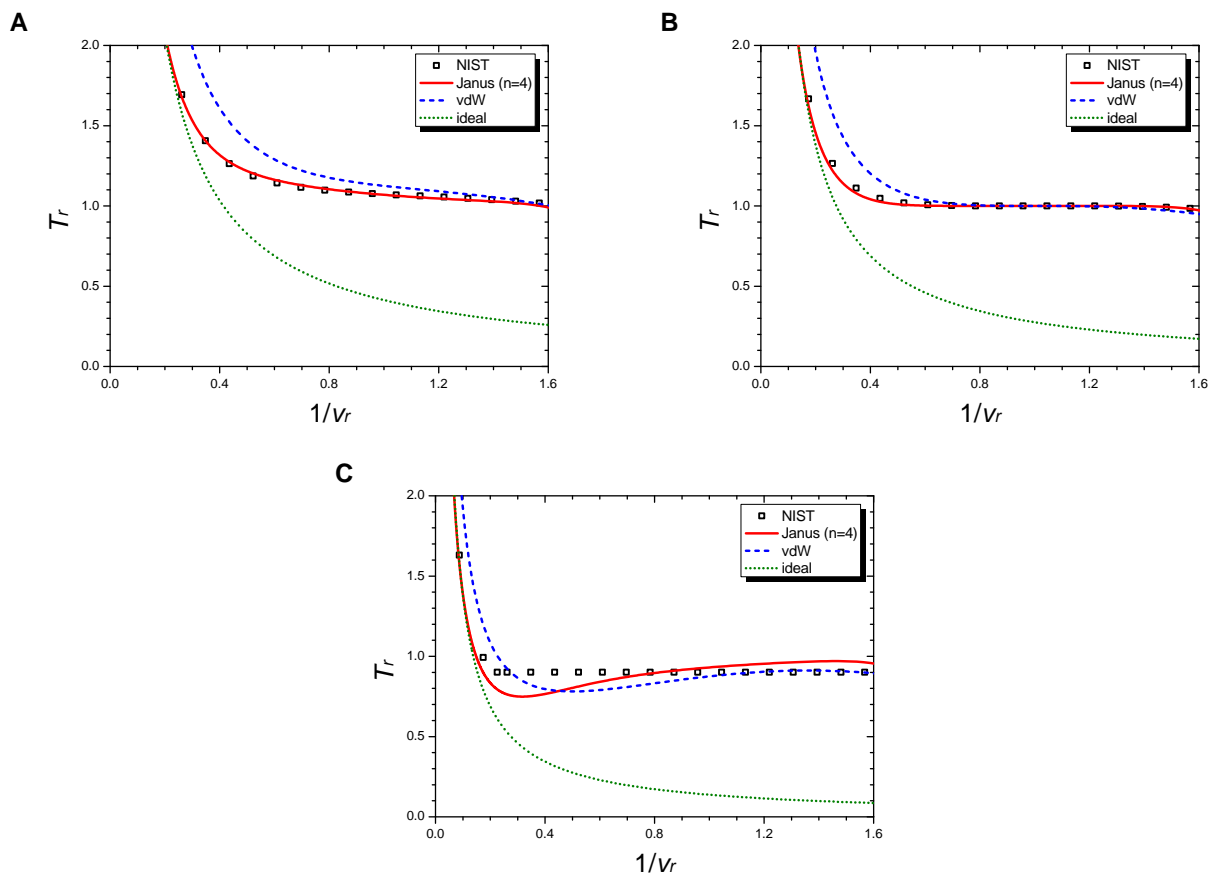

**Figure S18.** Isobaric curves of propylene ( $C_3H_6$ ) at  $P_r = 1.5$  (A),  $P_r = 1.0$  (B), and  $P_r = 0.5$  (C). Boxes are from the NIST data. The red solid line is drawn from the  $n = 4$  Janus van der Waals equation, the blue dashed line from the original van der Waals equation, and the green dotted line from the classical ideal gas law.

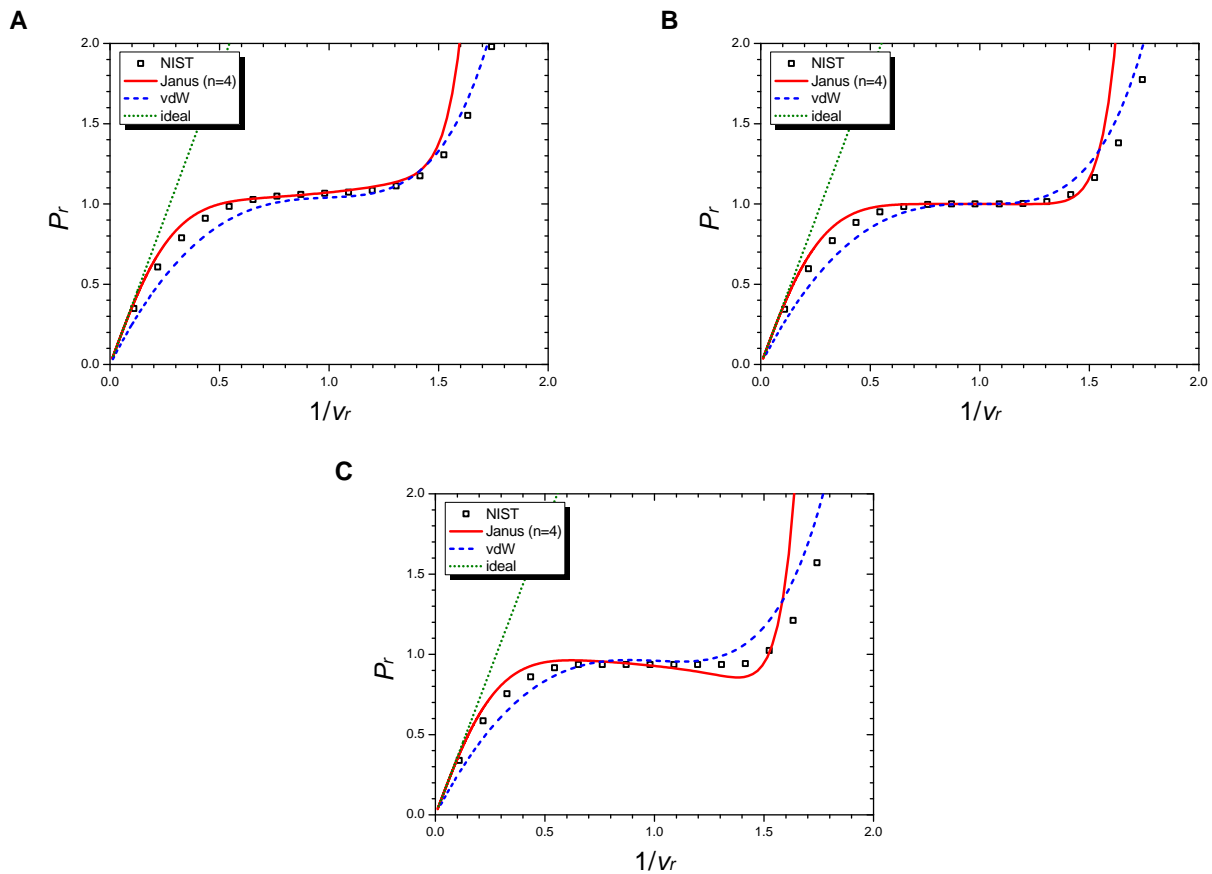

**Figure S19.** Isothermal curves of propylene ( $C_3H_6$ ) at  $T_r = 1.01$  (A),  $T_r = 1.00$  (B), and  $T_r = 0.99$  (C). Boxes are from the NIST data. The red solid line is drawn from the  $n = 4$  Janus van der Waals equation, the blue dashed line from the original van der Waals equation, and the green dotted line from the classical ideal gas law.

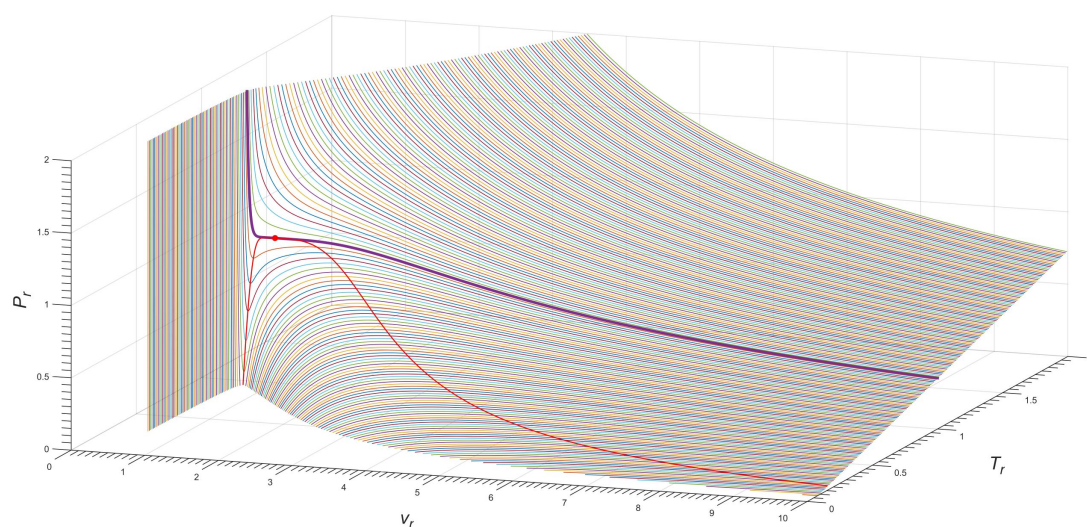

**Figure S20.** Three-dimensional  $P_r - v_r - T_r$  phase diagram of the exact  $n = 4$  Janus van der Waals equation, as for propylene ( $\text{C}_3\text{H}_6$ ). The bold purple line corresponds to the isotherm of  $T_r = 1.00$  as depicted in **Figure S19 B**; the red line is the Janus van der Waals spinodal curve with  $a = 0.99$ ; and the red dot is the critical point.



SM 1.6 propane ( $\text{C}_3\text{H}_8$ )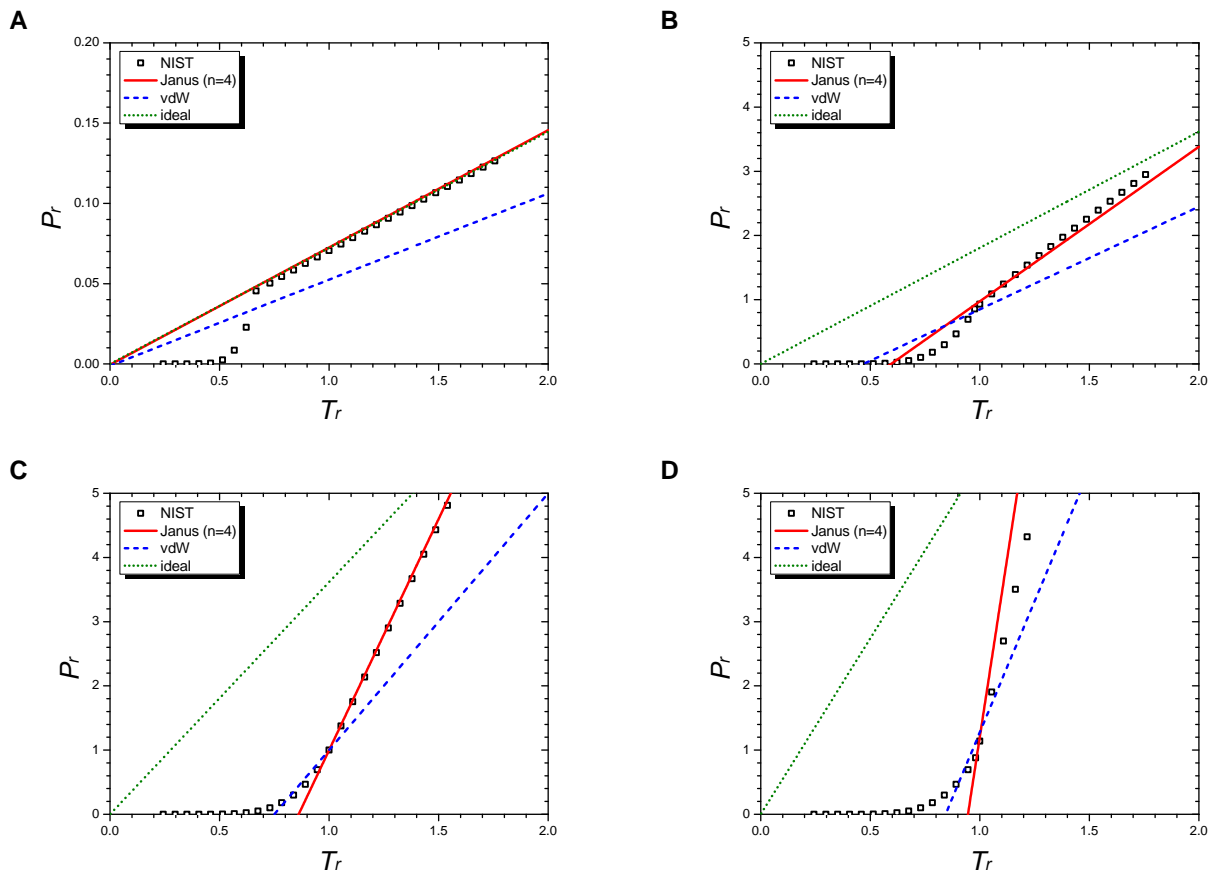

**Figure S21.** Isochoric curves of propane ( $\text{C}_3\text{H}_8$ ) at  $1/v_r = 0.02$  (A),  $1/v_r = 0.5$  (B),  $1/v_r = 1.0$  (C), and  $1/v_r = 1.5$  (D). Boxes are from the NIST data. The red solid line is drawn from the  $n = 4$  Janus van der Waals equation, the blue dashed line from the original van der Waals equation, and the green dotted line from the classical ideal gas law.

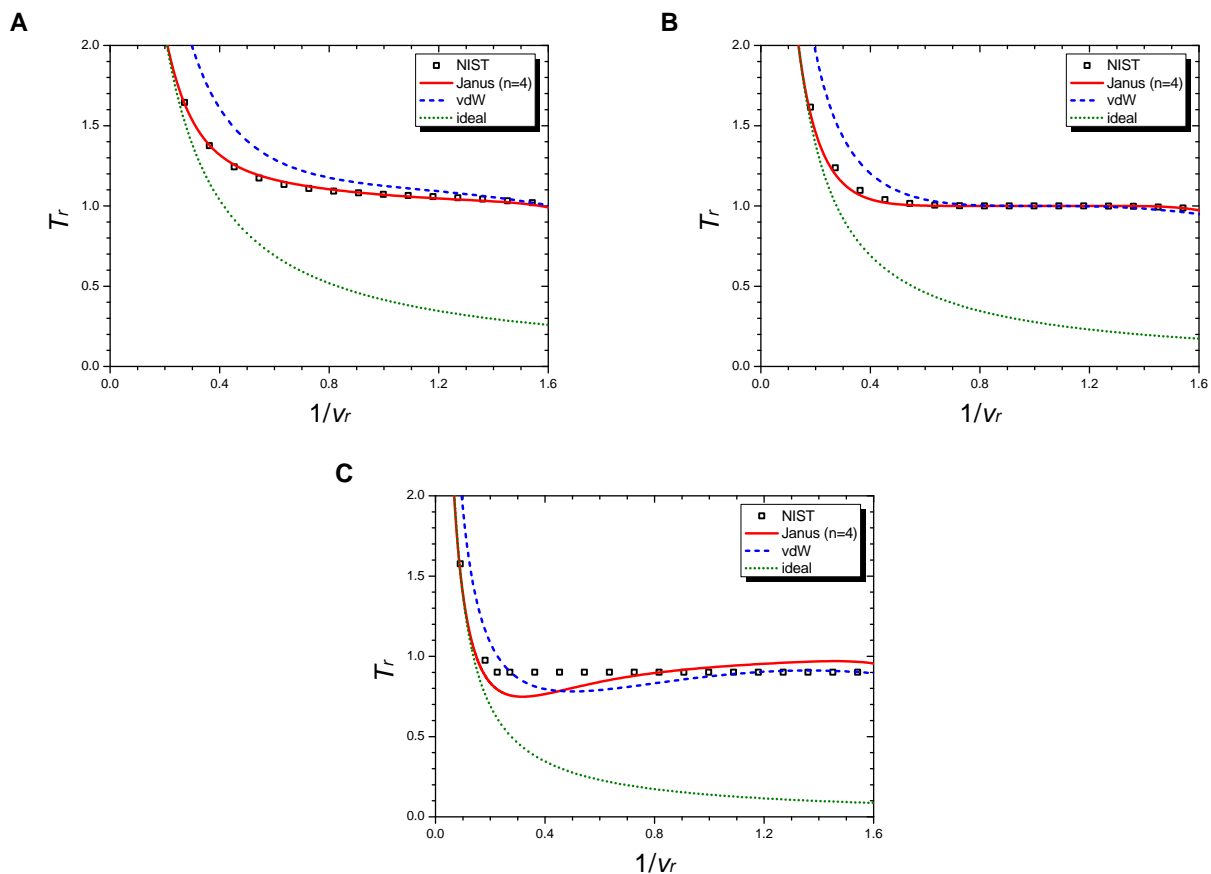

**Figure S22.** Isobaric curves of propane ( $C_3H_8$ ) at  $P_r = 1.5$  (A),  $P_r = 1.0$  (B), and  $P_r = 0.5$  (C). Boxes are from the NIST data. The red solid line is drawn from the  $n = 4$  Janus van der Waals equation, the blue dashed line from the original van der Waals equation, and the green dotted line from the classical ideal gas law.

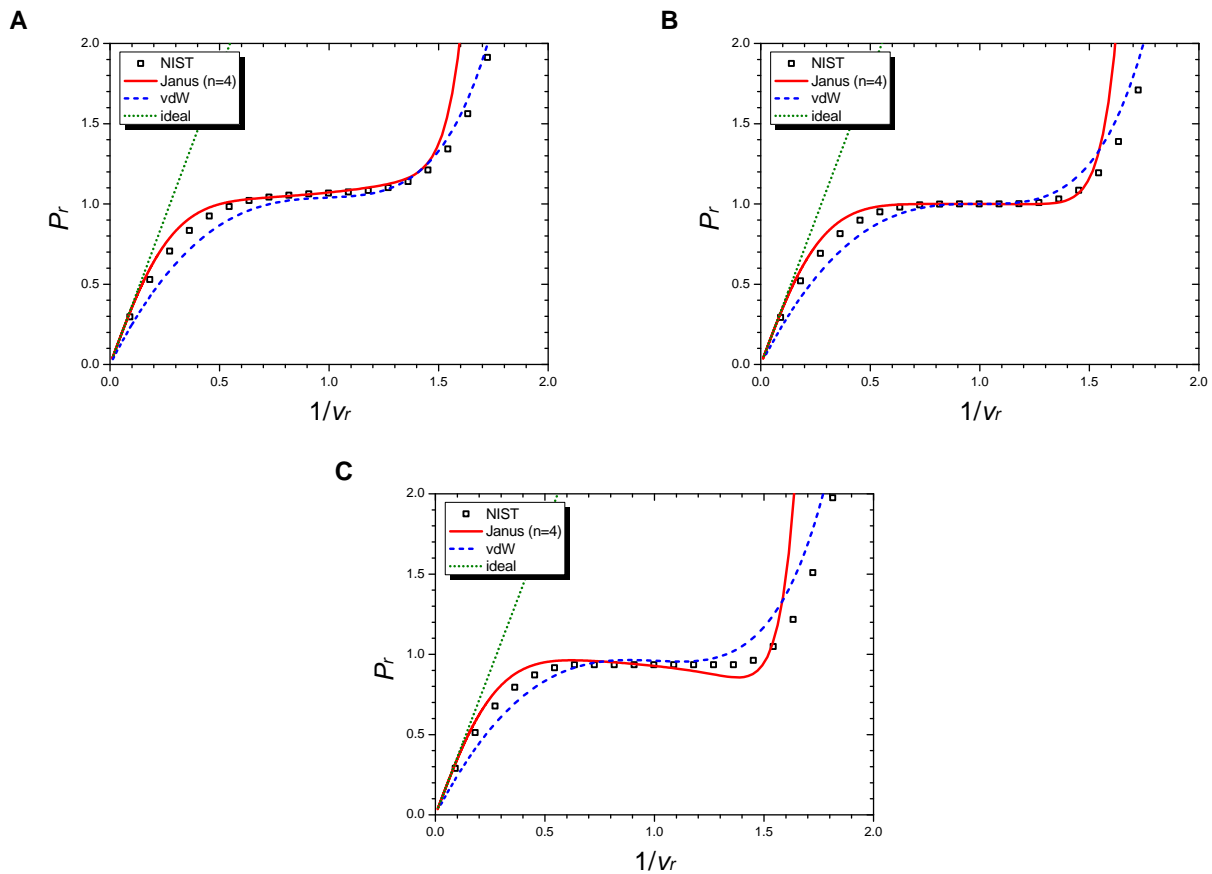

**Figure S23.** Isothermal curves of propane ( $\text{C}_3\text{H}_8$ ) at  $T_r = 1.01$  (A),  $T_r = 1.00$  (B), and  $T_r = 0.99$  (C). Boxes are from the NIST data. The red solid line is drawn from the  $n = 4$  Janus van der Waals equation, the blue dashed line from the original van der Waals equation, and the green dotted line from the classical ideal gas law.

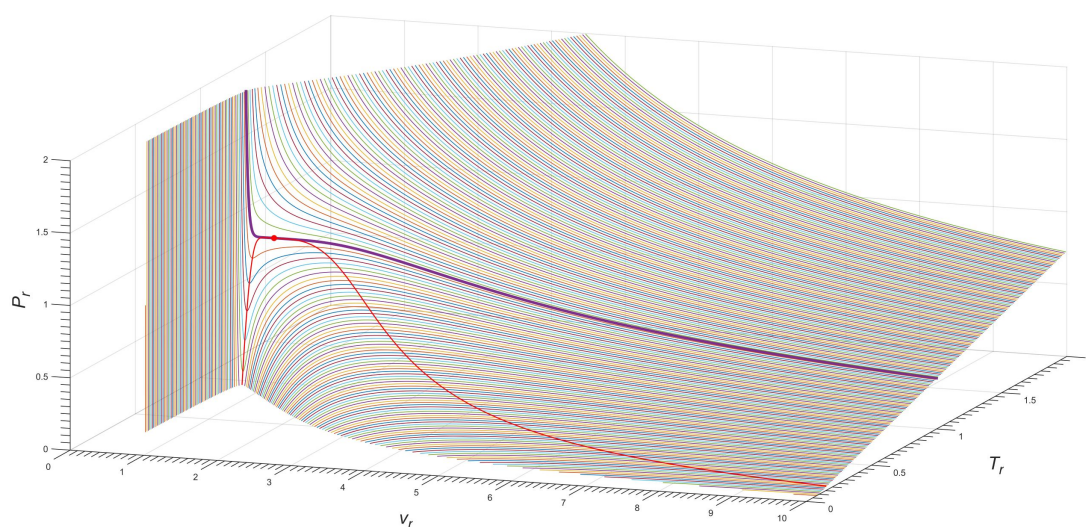

**Figure S24.** Three-dimensional  $P_r - v_r - T_r$  phase diagram of the exact  $n = 4$  Janus van der Waals equation, as for propane ( $\text{C}_3\text{H}_8$ ). The bold purple line corresponds to the isotherm of  $T_r = 1.00$  as depicted in **Figure S23 B**; the red line is the Janus van der Waals spinodal curve with  $a = 0.99$ ; and the red dot is the critical point.

SM 1.7 butane ( $\text{C}_4\text{H}_{10}$ )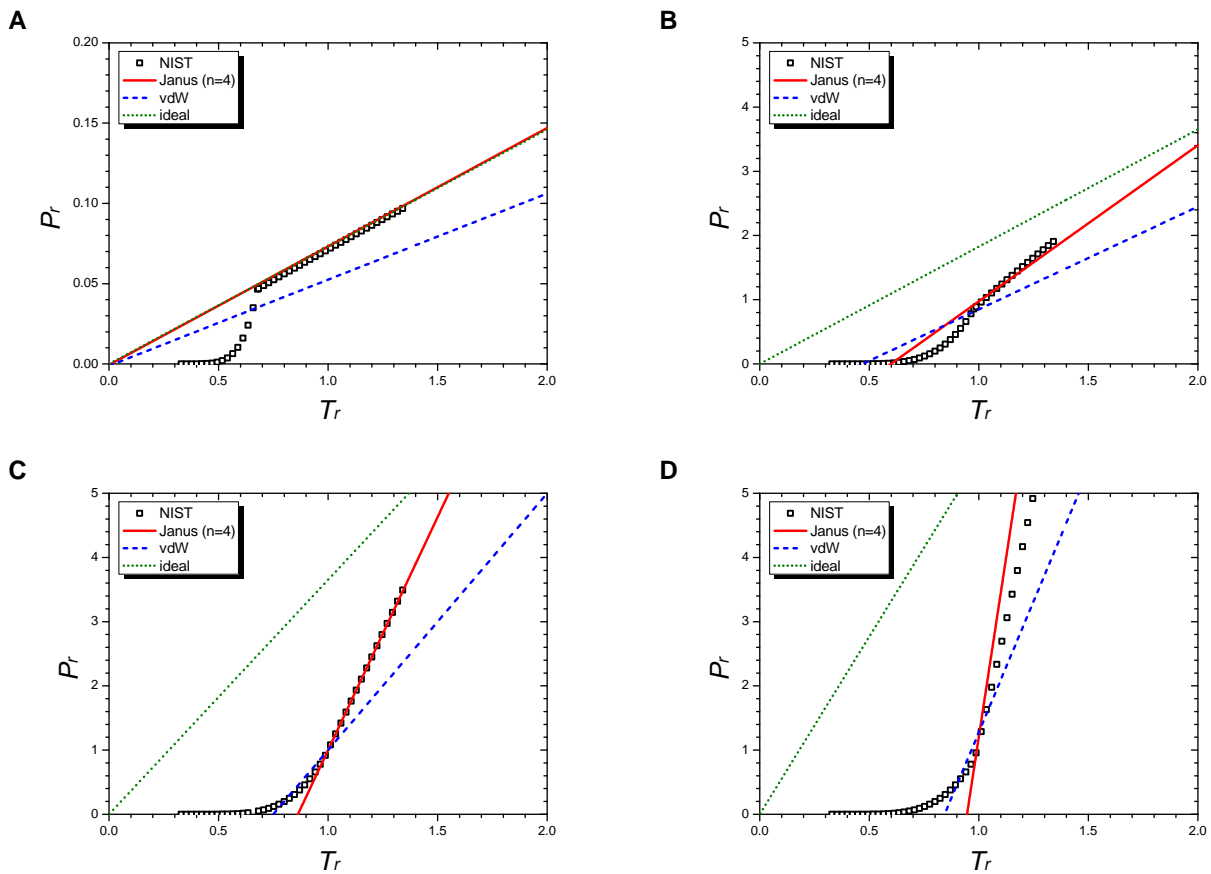

**Figure S25.** Isochoric curves of butane ( $\text{C}_4\text{H}_{10}$ ) at  $1/v_r = 0.02$  (A),  $1/v_r = 0.5$  (B),  $1/v_r = 1.0$  (C), and  $1/v_r = 1.5$  (D). Boxes are from the NIST data. The red solid line is drawn from the  $n = 4$  Janus van der Waals equation, the blue dashed line from the original van der Waals equation, and the green dotted line from the classical ideal gas law.

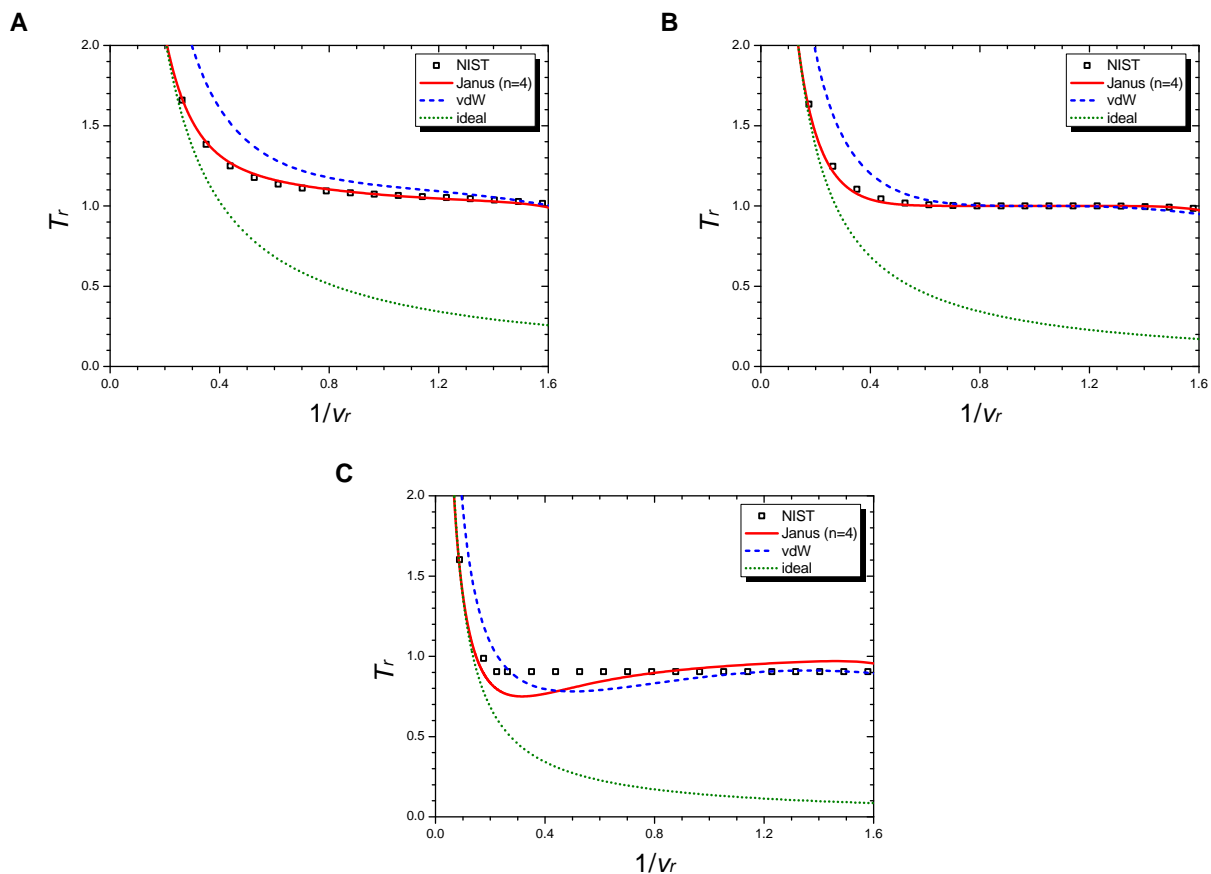

**Figure S26.** Isobaric curves of butane ( $C_4H_{10}$ ) at  $P_r = 1.5$  (A),  $P_r = 1.0$  (B), and  $P_r = 0.5$  (C). Boxes are from the NIST data. The red solid line is drawn from the  $n = 4$  Janus van der Waals equation, the blue dashed line from the original van der Waals equation, and the green dotted line from the classical ideal gas law.

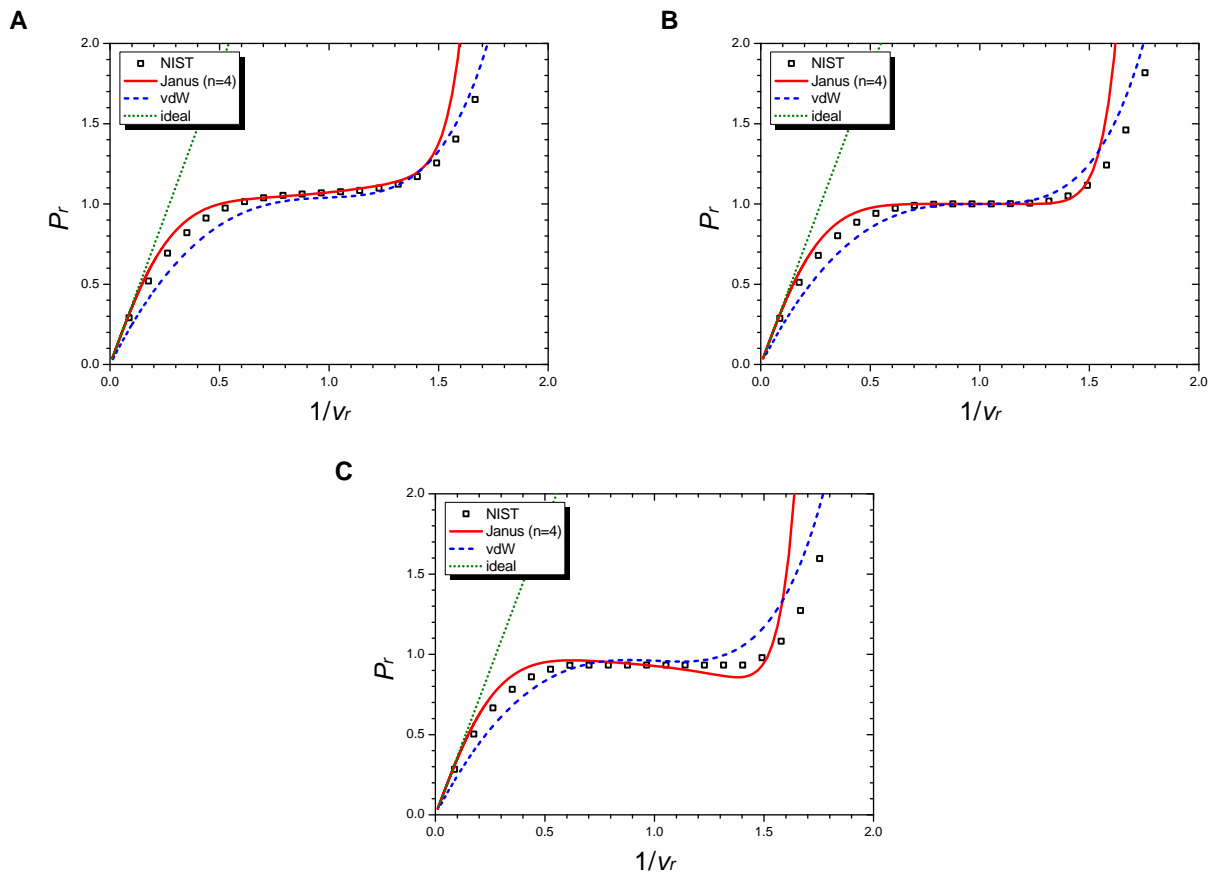

**Figure S27.** Isothermal curves of butane ( $C_4H_{10}$ ) at  $T_r = 1.01$  (A),  $T_r = 1.00$  (B), and  $T_r = 0.99$  (C). Boxes are from the NIST data. The red solid line is drawn from the  $n = 4$  Janus van der Waals equation, the blue dashed line from the original van der Waals equation, and the green dotted line from the classical ideal gas law.

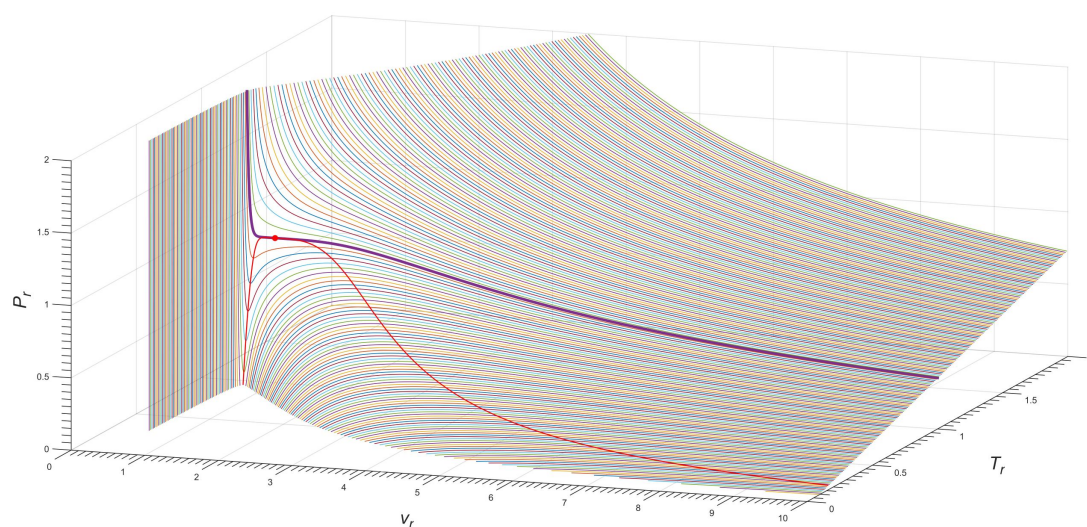

**Figure S28.** Three-dimensional  $P_r - v_r - T_r$  phase diagram of the exact  $n = 4$  Janus van der Waals equation, as for butane ( $\text{C}_4\text{H}_{10}$ ). The bold purple line corresponds to the isotherm of  $T_r = 1.00$  as depicted in **Figure S27 B**; the red line is the Janus van der Waals spinodal curve with  $a = 0.99$ ; and the red dot is the critical point.



SM 1.8 isobutane ( $\text{C}_4\text{H}_{10}$ )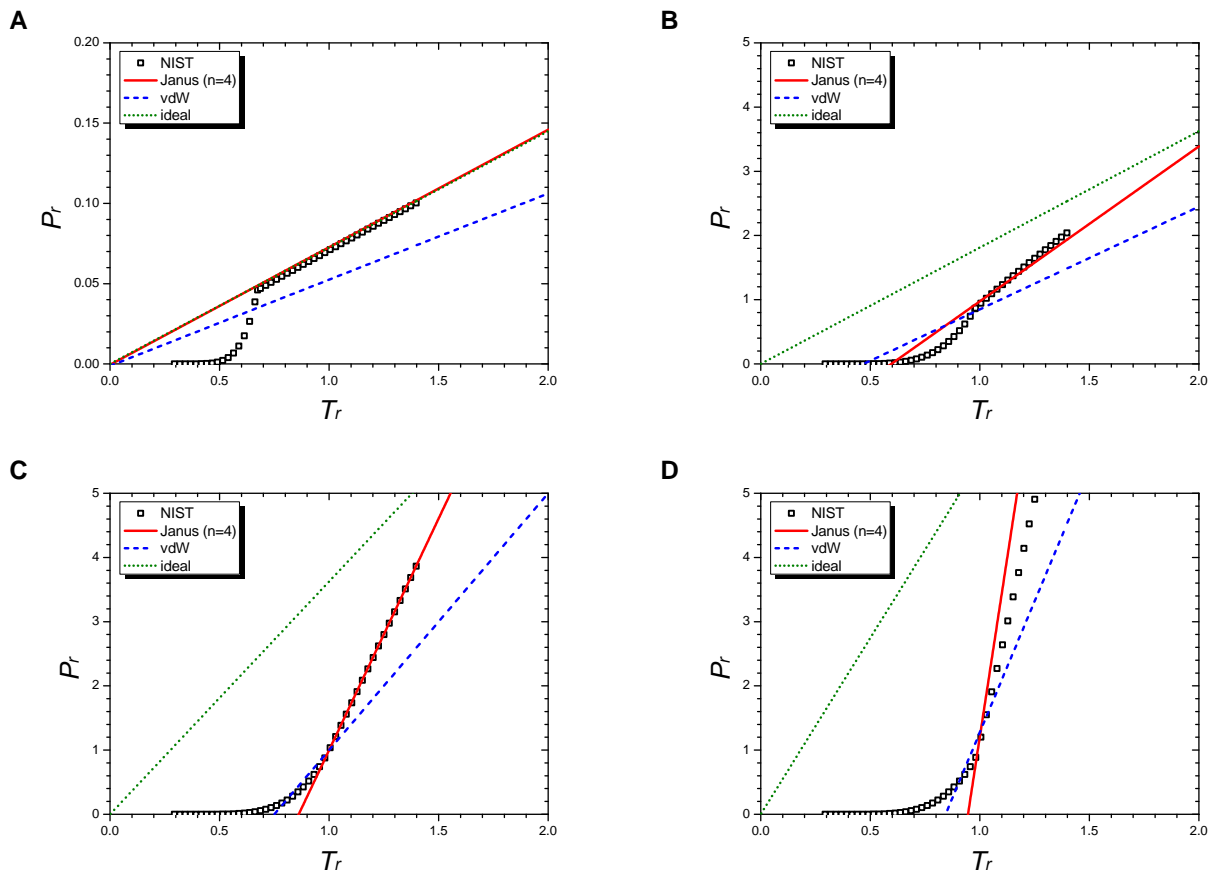

**Figure S29.** Isochoric curves of isobutane ( $\text{C}_4\text{H}_{10}$ ) at  $1/v_r = 0.02$  (A),  $1/v_r = 0.5$  (B),  $1/v_r = 1.0$  (C), and  $1/v_r = 1.5$  (D). Boxes are from the NIST data. The red solid line is drawn from the  $n = 4$  Janus van der Waals equation, the blue dashed line from the original van der Waals equation, and the green dotted line from the classical ideal gas law.

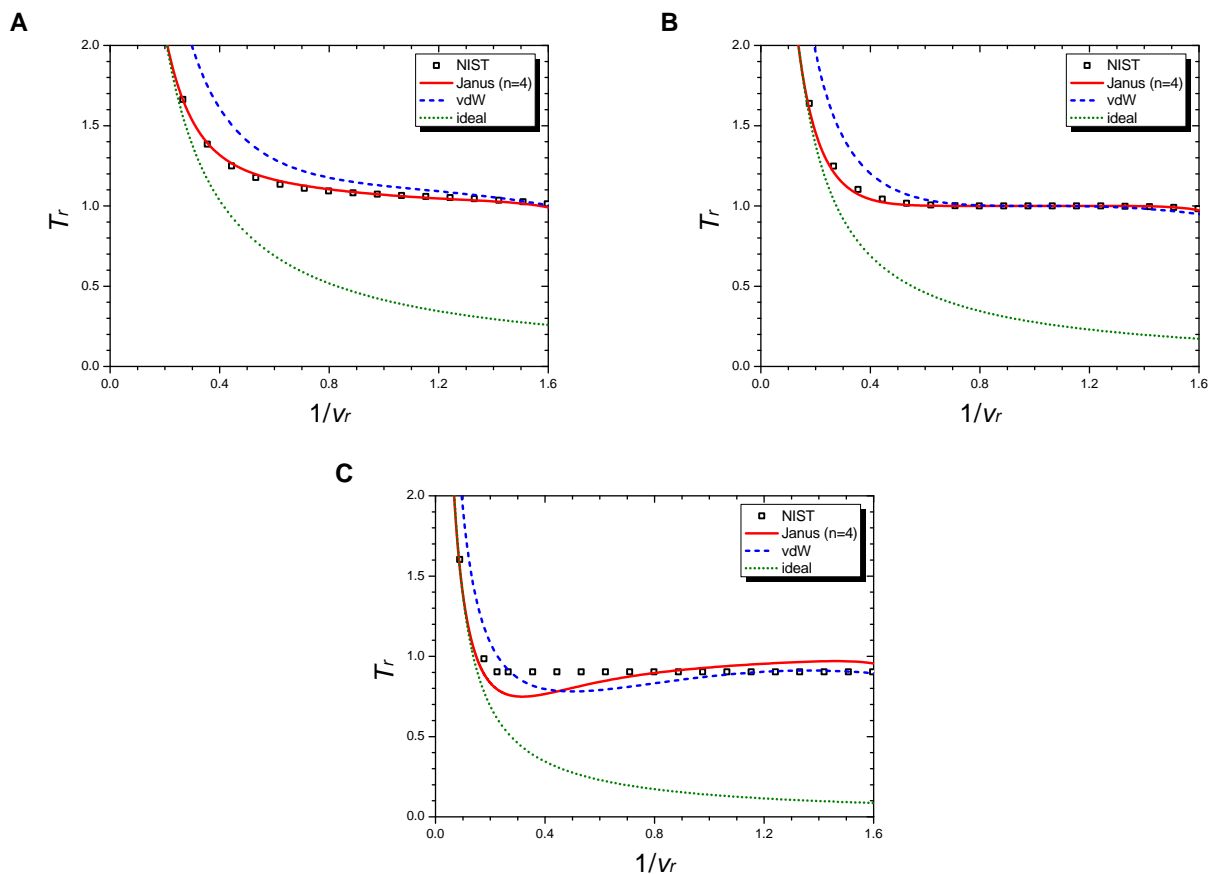

**Figure S30.** Isobaric curves of isobutane ( $C_4H_{10}$ ) at  $P_r = 1.5$  (A),  $P_r = 1.0$  (B), and  $P_r = 0.5$  (C). Boxes are from the NIST data. The red solid line is drawn from the  $n = 4$  Janus van der Waals equation, the blue dashed line from the original van der Waals equation, and the green dotted line from the classical ideal gas law.

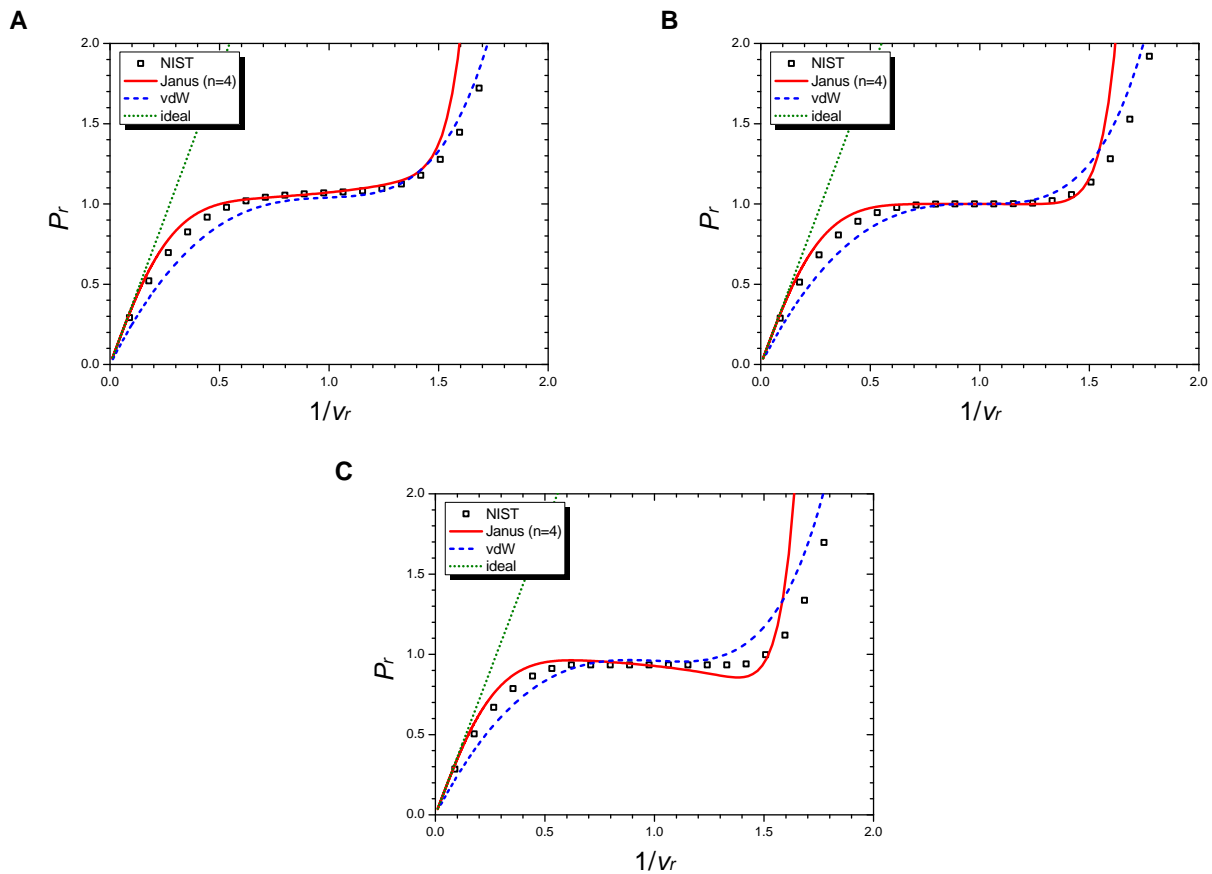

**Figure S31.** Isothermal curves of isobutane ( $C_4H_{10}$ ) at  $T_r = 1.01$  (A),  $T_r = 1.00$  (B), and  $T_r = 0.99$  (C). Boxes are from the NIST data. The red solid line is drawn from the  $n = 4$  Janus van der Waals equation, the blue dashed line from the original van der Waals equation, and the green dotted line from the classical ideal gas law.

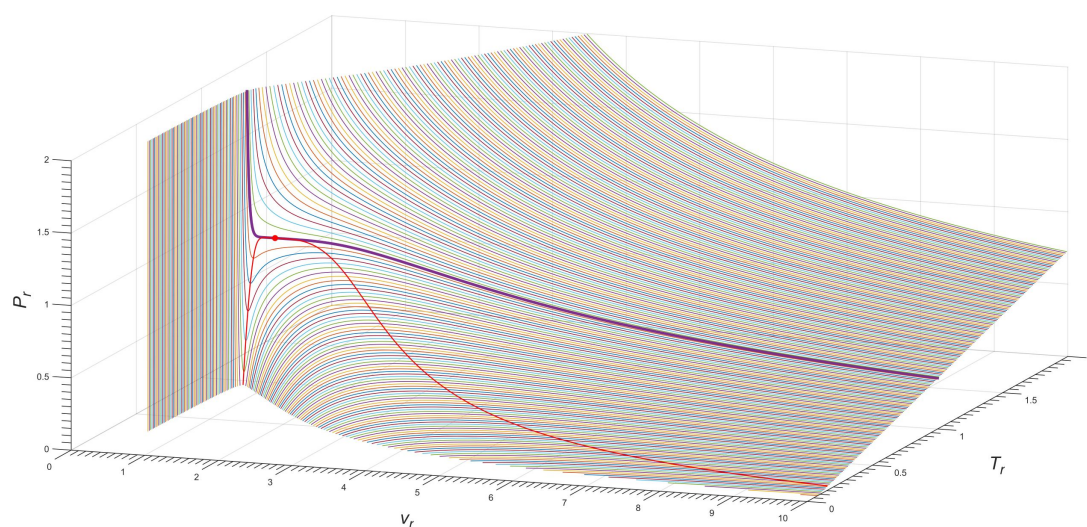

**Figure S32.** Three-dimensional  $P_r - v_r - T_r$  phase diagram of the exact  $n = 4$  Janus van der Waals equation, as for isobutane ( $\text{C}_4\text{H}_{10}$ ). The bold purple line corresponds to the isotherm of  $T_r = 1.00$  as depicted in **Figure S31 B**; the red line is the Janus van der Waals spinodal curve with  $a = 0.99$ ; and the red dot is the critical point.

SM 2 SUPPLEMENTARY FIGURES FOR  $N = 6$  CASEhelium-4 ( $^4\text{He}$ )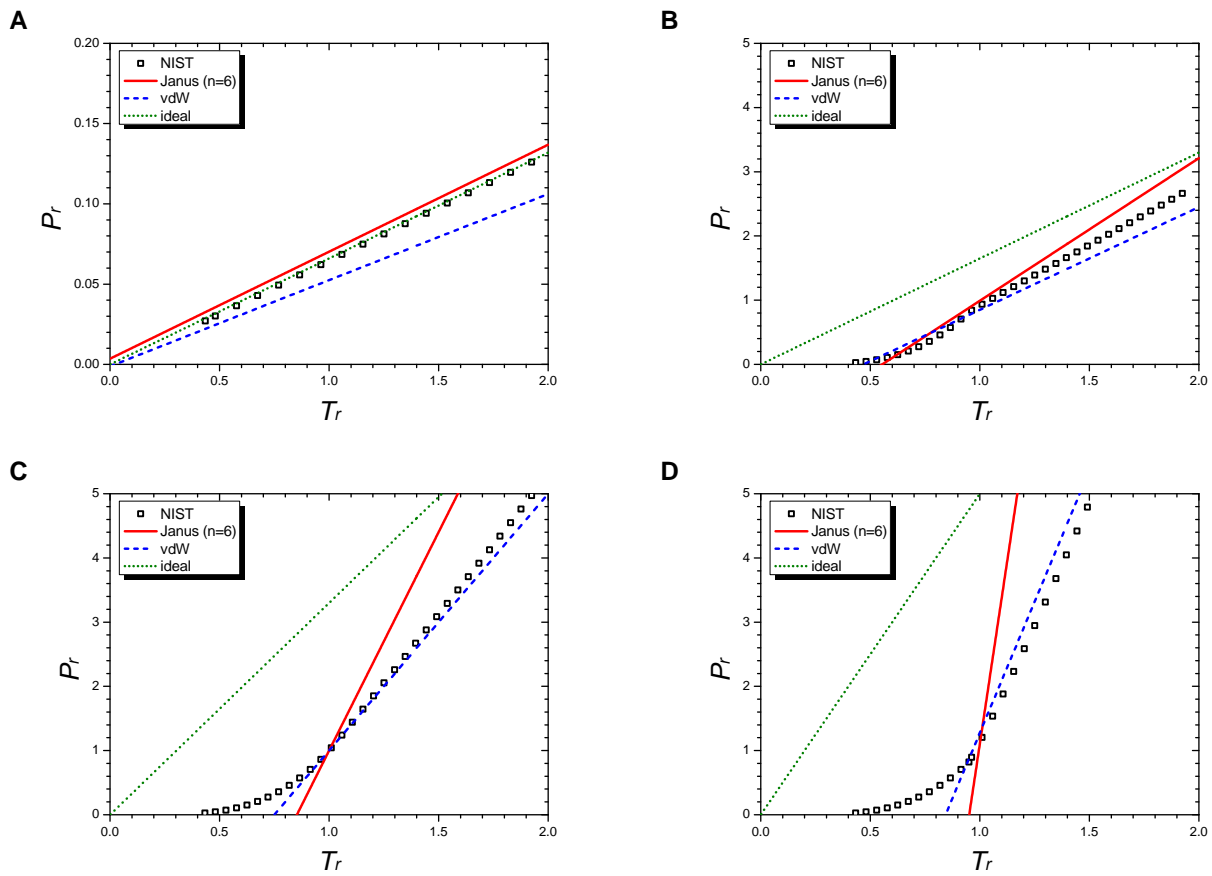

**Figure S33.** Isochoric curves of helium-4 ( $^4\text{He}$ ) at  $1/v_r = 0.02$  (A),  $1/v_r = 0.5$  (B),  $1/v_r = 1.0$  (C), and  $1/v_r = 1.5$  (D). Boxes are from the NIST data. The red solid line is drawn from the  $n = 6$  Janus van der Waals equation, the blue dashed line from the original van der Waals equation, and the green dotted line from the classical ideal gas law.

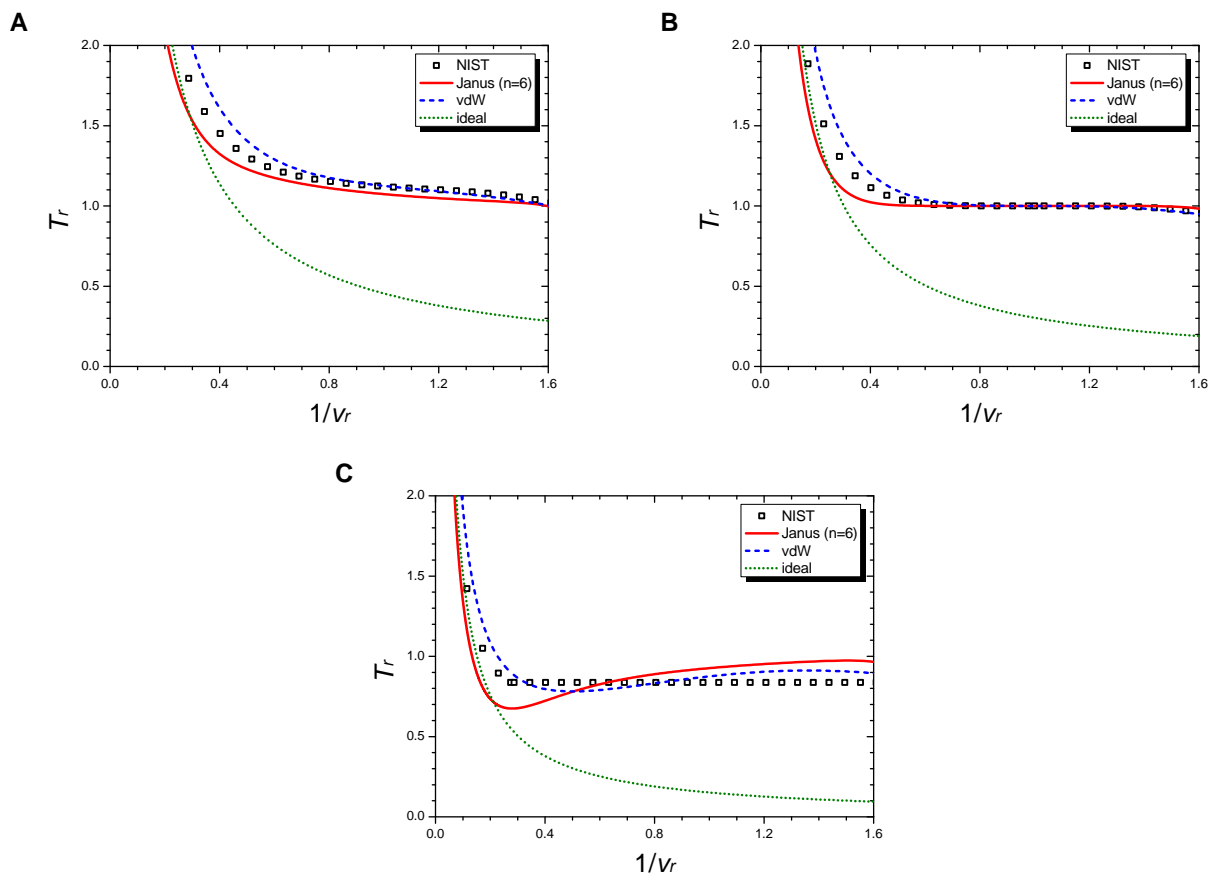

**Figure S34.** Isobaric curves of helium-4 ( ${}^4\text{He}$ ) at  $P_r = 1.5$  (A),  $P_r = 1.0$  (B), and  $P_r = 0.5$  (C). Boxes are from the NIST data. The red solid line is drawn from the  $n = 6$  Janus van der Waals equation, the blue dashed line from the original van der Waals equation, and the green dotted line from the classical ideal gas law.

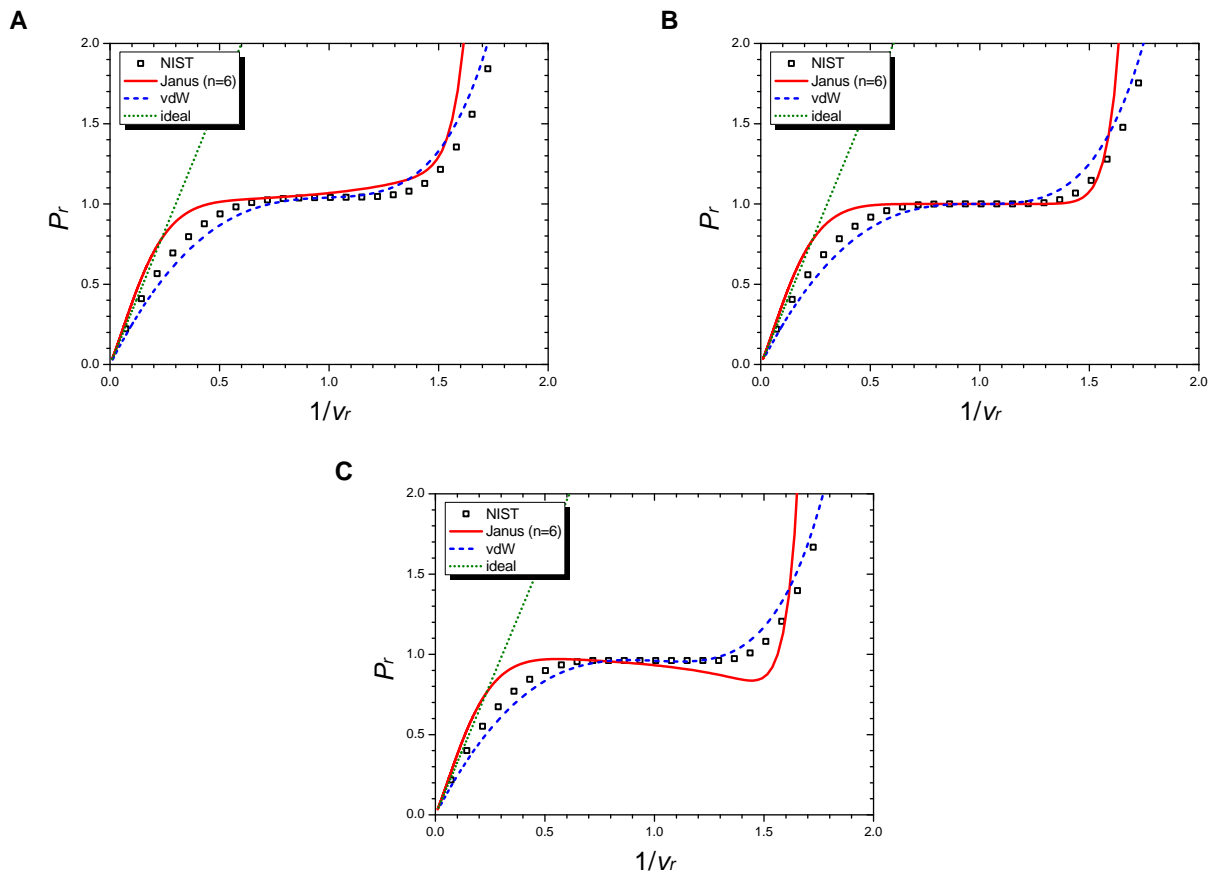

**Figure S35.** Isothermal curves of helium-4 ( $^4\text{He}$ ) at  $T_r = 1.01$  (A),  $T_r = 1.00$  (B), and  $T_r = 0.99$  (C). Boxes are from the NIST data. The red solid line is drawn from the  $n = 6$  Janus van der Waals equation, the blue dashed line from the original van der Waals equation, and the green dotted line from the classical ideal gas law.

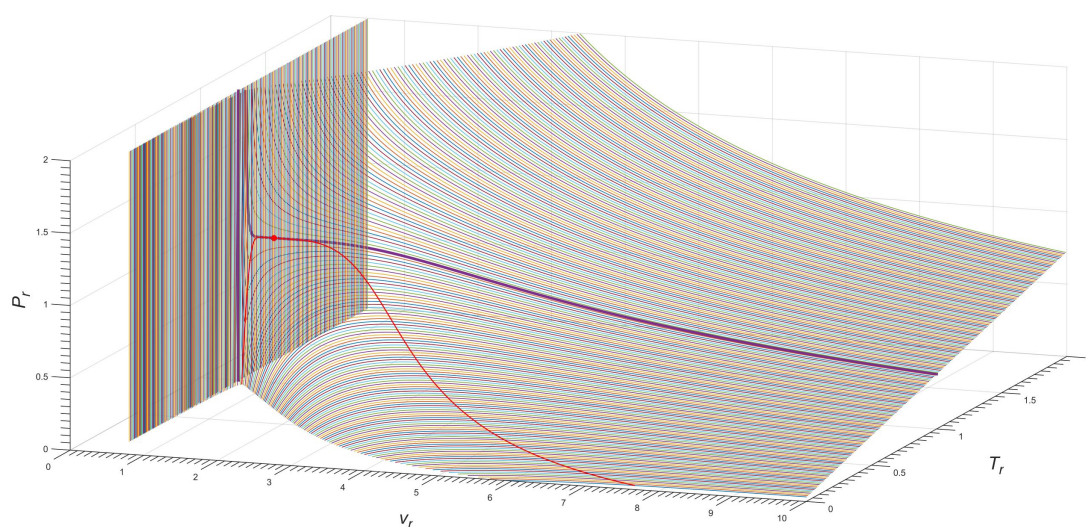

**Figure S36.** Three-dimensional  $P_r - v_r - T_r$  phase diagram of the exact  $n = 6$  Janus van der Waals equation, as for helium-4 ( $^4\text{He}$ ). The bold purple line corresponds to the isotherm of  $T_r = 1.00$  as depicted in **Figure S35 B**; the red line is the Janus van der Waals spinodal curve with  $a = 0.99$ ; and the red dot is the critical point.
